# Supplementary material for: Absolute vs Convective Instabilities and Front Propagation in Lipid Membrane Tubes
Source: arXiv:2008.13780 ancillary file (2022-02-12)
Supplement: Supplementary file 1 [file tchoufag-mandadapu-convective-SM.pdf]

# Supplemental Material
# Absolute/Convective Instabilities and Front Propagation in Lipid Membrane Tubes

Joël Tchoufag,[1,*] Amaresh Sahu,[1,‡] and Kranthi K. Mandadapu[1,2,†]

[1] Department of Chemical & Biomolecular Engineering, University of California, Berkeley, CA 94720, USA
[2] Chemical Sciences Division, Lawrence Berkeley National Laboratory, CA 94720, USA

## Contents

**I. Dynamics of lipid membrane tubes** **2**
1. General geometric and kinematic description . . . 2
2. General governing equations . . . 2
3. Axisymmetric governing equations . . . 3
   (a). Area parametrization . . . 3
   (b). Axial distance parametrization . . . 5
4. Linearized equations governing a lipid membrane tube . . . 6
   (a). Base state: Cylinder with constant axial velocity . . . 6
   (b). Perturbed equations and non-dimensionalization . . . 7
   (c). Axisymmetric evolution equation . . . 8

**II. Temporal stability analysis** **9**
1. Decomposition into normal modes . . . 9
2. Dispersion relation . . . 9
3. Linear stability analysis . . . 10

**III. Spatiotemporal stability analysis** **11**
1. Saddle points of the dispersion relation . . . 12
   (a). Purely imaginary absolute wavenumber . . . 13
   (b). Absolute wavenumber with nonzero real and imaginary parts . . . 14
2. Absolute to convective transition . . . 15
3. Limiting behavior of $SL_{\mathrm{ac}}$ . . . 19
   (a). Limiting behavior when $\Gamma$ is large . . . 19
   (b). Limiting behavior when $\Gamma$ approaches $\Gamma_{\mathrm{c}}$ . . . 19
4. Numerical solutions of linearized dynamics . . . 20
5. Speed of propagating fronts: Marginal stability criterion . . . 22
6. Understanding $\Gamma_1$ and $\Gamma_2$ as Lifshitz points . . . 23

**IV. Nonlinear dynamics** **24**
1. Weakly nonlinear analysis . . . 24
2. Weakly vs. fully nonlinear simulations . . . 27
   (a). Inward localized perturbation . . . 28
   (b). Outward localized perturbation . . . 30
   (c). Global perturbation . . . 33
3. Final observations . . . 36

**References** **37**

*jtchoufa@berkeley.edu
‡amaresh.sahu@berkeley.edu
†kranthi@berkeley.edu

# I. Dynamics of lipid membrane tubes

In this section, we present the dynamical equations governing an unperturbed and perturbed lipid membrane tube. We first describe the geometry and kinematics of an arbitrarily curved and deforming lipid membrane, and then provide the corresponding equations of motion. Next, the equations are specialized to the case of an axisymmetric membrane, which can undergo arbitrarily large deformations. Finally, we obtain the linearized dynamical equations governing unperturbed and perturbed lipid membrane tubes, which have a constant axial base flow prior to being perturbed. A dimensional analysis of the perturbed equations reveals membrane dynamics are governed by two dimensionless numbers: the well-known Föppl–von Kármán number $\Gamma$, and the recently introduced Scriven–Love number $SL$ [1].

## 1. General geometric and kinematic description

We begin by describing the geometry of an arbitrarily curved membrane, which is modeled as a single two-dimensional differentiable manifold. In describing the membrane as such, it is implicitly assumed that there is no slip between the two bilayer leaflets. While only relevant geometric concepts are highlighted below, more details can be found in our previous work [2, Sec. II] and the references provided therein.

The position of the membrane surface $\boldsymbol{x}$ is parametrized by two general coordinates $\theta^1$ and $\theta^2$, as well as the time $t$, written as $\boldsymbol{x} = \boldsymbol{x}(\theta^\alpha, t)$. Here and henceforth, Greek indices span the set $\{1, 2\}$; moreover, the Einstein summation is employed, in which Greek indices repeated in a subscript and superscript are summed over. At any point $\boldsymbol{x}$, we define the vectors $\boldsymbol{a}_\alpha := \partial \boldsymbol{x}/\partial \theta^\alpha = \boldsymbol{x}_{,\alpha}$ spanning the tangent plane to the surface, as well as the unit normal $\boldsymbol{n} := (\boldsymbol{a}_1 \times \boldsymbol{a}_2)/|\boldsymbol{a}_1 \times \boldsymbol{a}_2|$. The set $\{\boldsymbol{a}_\alpha, \boldsymbol{n}\}$ is a basis of $\mathbb{R}^3$, such that any vector $\boldsymbol{u} \in \mathbb{R}^3$ can be decomposed as $\boldsymbol{u} = u^\alpha \boldsymbol{a}_\alpha + u\boldsymbol{n}$. Distances on the membrane surface are captured by the covariant metric $a_{\alpha\beta} := \boldsymbol{a}_\alpha \cdot \boldsymbol{a}_\beta$ and its matrix inverse, the contravariant metric $a^{\alpha\beta}$. With the metric, as well as the curvature components $b_{\alpha\beta} := \boldsymbol{n} \cdot \boldsymbol{x}_{,\alpha\beta}$, the mean curvature $H$ and Gaussian curvature $K$ are found according to $H := \frac{1}{2} a^{\alpha\beta} b_{\alpha\beta}$ and $K := \det(b_{\alpha\beta})/\det(a_{\alpha\beta})$. The covariant and contravariant metric are additionally used to lower and raise indices, respectively.

Consider the in-plane components $u^\alpha$ of a general vector $\boldsymbol{u}$. On a curved surface, the partial derivative of $u^\alpha$ with respect to the coordinate $\theta^\beta$, denoted $u^\alpha_{,\beta}$, will in general not transform as a tensor under a change in the surface parametrization. We define the covariant derivative of $u^\alpha$ with respect to $\theta^\beta$, denoted $u^\alpha_{;\beta}$, to transform as the components of a tensor under a change in parametrization of the surface. The covariant derivative $u^\alpha_{;\beta}$ is calculated as $u^\alpha_{;\beta} = u^\alpha_{,\beta} + \Gamma^\alpha_{\beta\mu} u^\mu$, where the Christoffel symbols $\Gamma^\alpha_{\beta\mu}$ are given by $\Gamma^\alpha_{\beta\mu} := \frac{1}{2} a^{\alpha\delta}(a_{\delta\beta,\mu} + a_{\delta\mu,\beta} - a_{\beta\mu,\delta})$.

Thus far, we described the geometry of a surface at a single instant in time, however in general lipid membranes deform over time and a kinematic description of their motion is required. The velocity $\boldsymbol{v}$ of the membrane is the material time derivative of its position, written as $\boldsymbol{v} := \mathrm{d}\boldsymbol{x}/\mathrm{d}t = \dot{\boldsymbol{x}}$ and expanded in the $\{\boldsymbol{a}_\alpha, \boldsymbol{n}\}$ basis as $\boldsymbol{v} = v^\alpha \boldsymbol{a}_\alpha + v\boldsymbol{n}$. Moreover, the surface parametrization $\theta^\alpha$ is chosen such that a point of constant $\theta^\alpha$ only moves normal to the membrane surface, for which $v\boldsymbol{n} = (\boldsymbol{v} \cdot \boldsymbol{n})\boldsymbol{n} = (\partial \boldsymbol{x}/\partial t)|_{\theta^\alpha}$ and $v^\alpha = \dot{\theta}^\alpha$. We additionally find $\dot{\boldsymbol{a}} = \boldsymbol{v}_{,\alpha}$ and $\dot{a}_{\alpha\beta} = v_{\alpha;\beta} + v_{\beta;\alpha} - 2vb_{\alpha\beta}$.

## 2. General governing equations

Lipid membranes have a unique constitutive behavior: lipids flow in-plane as a two-dimensional viscous fluid, and the membrane bends elastically out-of-plane [3]. In this section, we present the equations governing membrane dynamics, obtained via a balance law formulation in which the membrane stresses were obtained with techniques from irreversible thermodynamics—all within a differential geometric setting (see Ref. [2] for full details).

To begin, lipid membranes can only stretch 2–3% before tearing [3], and are thus modeled as being area-incompressible. A local mass balance yields the continuity equation

$$v^\alpha_{;\alpha} \, - \, 2vH \, = \, 0 \; . \tag{1}$$

The incompressibility constraint of Eq. (1) is enforced by the Lagrange multiplier $\lambda = \lambda(\theta^\alpha, t)$, which physically acts as the membrane tension. Importantly, the tension is not constant, but at every point takes the requisite value to enforce Eq. (1); it is also equivalently the negative surface pressure.

We next present the in-plane and out-of-plane components of the linear momentum balance. The in-plane equations are given by

$$0 \;=\; \big(\lambda\, a^{\alpha\beta} \,+\, \pi^{\beta\alpha}\big)_{;\beta} \;=\; a^{\alpha\beta}\lambda_{,\beta} \,+\, \pi^{\beta\alpha}_{;\beta} ~, \tag{2}$$

where

$$\pi^{\alpha\beta} \;=\; \zeta\,\dot{a}_{\mu\nu}\,a^{\alpha\mu}\,a^{\beta\nu} \tag{3}$$

are the in-plane viscous stresses, $(\lambda a^{\alpha\beta} + \pi^{\alpha\beta})$ are the total in-plane fluid stresses, and $\zeta$ is the two-dimensional intramembrane viscosity. Physically, Eq. (2) indicates surface tension gradients drive an in-plane flow of lipids, in a similar manner to how pressure gradients drive flows in bulk three-dimensional fluids. Equation (2) is identical to the equation governing the in-plane dynamics of a two-dimensional fluid film [4,5]. We note that inertial terms are not included, as they are negligible in both the in-plane and out-of-plane dynamics [1].

The out-of-plane equation of motion, also called the shape equation, is given by

$$0 \;=\; p \,+\, 2\lambda H \,+\, \pi^{\alpha\beta} b_{\alpha\beta} \,-\, 2k_{\mathrm{b}}\, H\big(H^2 - K\big) \,-\, k_{\mathrm{b}}\,\Delta_{\mathrm{s}} H ~. \tag{4}$$

In Eq. (4), $p$ is the jump in normal stress across the membrane, which for example could be due to hydrodynamic or osmotic pressure drops in the surrounding fluid. In this work, however, the dynamics of the surrounding fluid are not taken into account and $p$ is treated as a constant. Additionally, in Eq. (4) $k_{\mathrm{b}}$ is the bending modulus of the membrane, with units of energy, and $\Delta_{\mathrm{s}}$ is the surface Laplacian—defined as $\Delta_{\mathrm{s}}(\,\cdot\,) := a^{\alpha\beta}(\,\cdot\,)_{;\alpha\beta}$. In the limit of a static membrane with no bending modulus, Eq. (4) simplifies to the Young–Laplace equation $p + 2\lambda H = 0$; moreover, bending terms involving $k_{\mathrm{b}}$ are expected as the membrane bends elastically out-of-plane. The $\pi^{\alpha\beta} b_{\alpha\beta}$ term contains the in-plane viscous shear stresses and membrane curvature, and arises from the coupling between in-plane and out of-plane membrane dynamics—discussed extensively in Ref. [1].

Equations (1)–(4) are the four equations required to solve for the four fundamental membrane unknowns: the surface tension $\lambda$, and the three components of the membrane velocity $\boldsymbol{v}$. However, though the general equations are known, they are complex to solve both analytically and numerically. In the remainder of this section, we provide a simplified form of the governing equations in different circumstances, all of which are useful in obtaining our later results.

## 3. Axisymmetric governing equations

When analyzing the dynamics and stability of membrane tubes, we will find in Sec. II that it is useful to consider axisymmetric geometries—namely, those that are rotationally symmetric about an axis. The symmetry axis is chosen to coincide with the $z$-axis of a standard Cartesian coordinate system, such that the azimuthal angle $\theta$ is measured in the $x$–$y$ plane. In what follows, we present the equations governing lipid membrane dynamics for two choices of surface parametrization in an axisymmetric setting.

### (a). Area parametrization

As shown in Fig. 1, the $z$-axis is the axis of rotational symmetry and $r$ is the distance from the $z$-axis, such that any axisymmetric surface can be described by a curve in the $r$–$z$ plane. Just as a curve can be parametrized by its arclength $s$, we follow Refs. [6,7] and parametrize an axisymmetric membrane surface by its area $a$. With rotational symmetry about the $z$-axis, we have

$$\mathrm{d}a \;=\; 2\pi r\sqrt{\mathrm{d}r^2 \,+ \mathrm{d}z^2} ~, \tag{5}$$

such that we can define an angle $\varphi$ satisfying

$$\frac{\mathrm{d}r}{\mathrm{d}a} \;=\; \frac{\cos\varphi}{2\pi r} \qquad \text{and} \qquad \frac{\mathrm{d}z}{\mathrm{d}a} \;=\; \frac{\sin\varphi}{2\pi r} ~, \tag{6}$$

as depicted in Fig. 1. We parametrize the surface position as

$$\boldsymbol{x}(\theta, a, t) \;=\; r(a,t)\,\boldsymbol{e}_r(\theta) \,+\, z(a,t)\,\boldsymbol{e}_z ~, \tag{7}$$

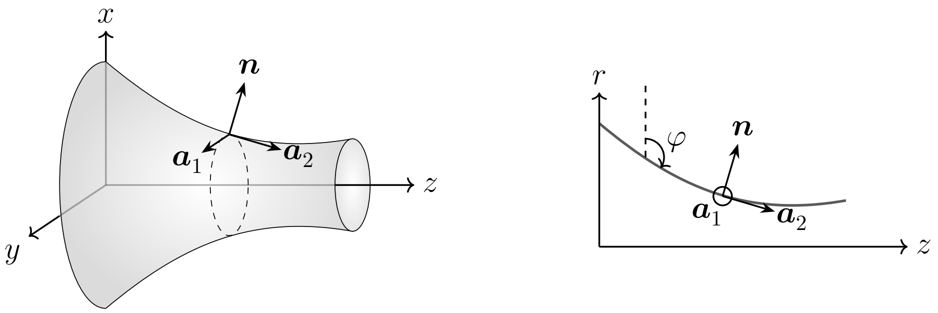


Figure 1: Schematic of an axisymmetric surface of revolution (a), and its representation as a curve in the $r$–$z$ plane (b). In both cases, the basis vectors $\boldsymbol{a}_1$, $\boldsymbol{a}_2$, and $\boldsymbol{n}$ are shown. The angle $\varphi$ depicted in (b) is introduced for notational and computational convenience.

and calculate the basis vectors to be given by

$$\boldsymbol{a}_1 = r\boldsymbol{e}_\theta , \qquad \boldsymbol{a}_2 = \frac{\cos\varphi}{2\pi r}\boldsymbol{e}_r + \frac{\sin\varphi}{2\pi r}\boldsymbol{e}_z , \qquad \text{and} \qquad \boldsymbol{n} = \sin\varphi\,\boldsymbol{e}_r - \cos\varphi\,\boldsymbol{e}_z . \tag{8}$$

Note that in order to be consistent with our previous theoretical developments [1, 2], the basis vectors $\boldsymbol{a}_1$ and $\boldsymbol{a}_2$ were chosen such that the unit normal $\boldsymbol{n}$ points outwards. In contrast, our past discussion of an area parametrization [7] had an inward pointing normal. Thus, though the results of this section are contained in the Supplementary Information of Ref. [7], our expressions differ slightly given the choice of basis vectors. With this in mind, we calculate the metric and curvature tensors as

$$a_{\alpha\beta} = \operatorname{diag}\Big(r^2,\, (2\pi r)^{-2}\Big) \qquad \text{and} \qquad b_{\alpha\beta} = -\operatorname{diag}\Big(r\sin\varphi,\, \varphi'/(2\pi r)\Big) . \tag{9}$$

In Eq. (9) and from now on, we use the notation $(\,\cdot\,)' := (\,\cdot\,)_{,a}$ to denote partial differentiation with respect to the area coordinate $a$; as we assume axisymmetry, the partial derivative of any quantity with respect to $\theta$ is zero. With the metric and curvature components, we calculate the mean and Gaussian curvature as

$$H = -\frac{1}{2}\Big(2\pi r\,\varphi' + \frac{1}{r}\sin\varphi\Big) \qquad \text{and} \qquad K = 2\pi\sin\varphi\,\varphi' . \tag{10}$$

Finally, the nonzero Christoffel symbols are found to be

$$\Gamma^2_{11} = -2\pi r^2\cos\varphi , \qquad \Gamma^1_{21} = \Gamma^1_{12} = \frac{\cos\varphi}{2\pi r^2} , \qquad \text{and} \qquad \Gamma^2_{22} = -\frac{\cos\varphi}{2\pi r^2} . \tag{11}$$

At this point, we substitute the geometric quantities obtained in Eqs. (5)–(11) into the general governing equations (1)–(4). We denote $u := v^a$ to be the in-plane velocity for notational convenience, and recognize the out-of-plane velocity $v = \boldsymbol{v}\cdot\boldsymbol{n}$ is given by

$$v = \sin\varphi\, r_{,t} - \cos\varphi\, z_{,t} , \tag{12}$$

where $(\,\cdot\,)_{,t}$ denotes the partial derivative with respect to time. The continuity, in-plane, and shape equations are then respectively given by [7]

$$u' - 2vH = 0 , \tag{13}$$

$$\zeta\sin\varphi\left[\frac{\varphi' u}{\pi r^2} - \frac{2}{r}v'\right] + \lambda' = 0 , \tag{14}$$

and

$$\begin{aligned} &p + 2\lambda H - 2k_{\mathrm{b}}H\big(H^2 - K\big) - k_{\mathrm{b}}\Big(4\pi\cos\varphi\, H' + 4\pi^2 r^2 H''\Big) \\ &\quad + 2\zeta\Big(-4\pi r v\varphi' H + \varphi' r^{-1} u\cos\varphi - \sin\varphi\cos\varphi\,(2\pi r^3)^{-1} u - 2v\big(2H^2 - K\big)\Big) = 0 , \end{aligned} \tag{15}$$

where the continuity equation (13) was used to simplify both the in-plane (14) and shape (15) equations. By defining the quantity

$$L \;:=\; k_{\mathrm{b}}\, 2\pi r^2\, H' \tag{16}$$

such that the fourth term in Eq. (15) can be written as $-2\pi L'$ and introducing an auxiliary variable for the in-plane velocity gradient

$$w \;:=\; u' \;, \tag{17}$$

the three governing equations (13–15) can be written as a system of eight first-order ordinary differential equations, given by [7]

$$r' \;=\; \frac{\cos\varphi}{2\pi r} \;, \tag{18}$$

$$z' \;=\; \frac{\sin\varphi}{2\pi r} \;, \tag{19}$$

$$\varphi' \;=\; \frac{-1}{2\pi r}\Big(2H \,+\, \frac{1}{r}\,\sin\varphi\Big) \;, \tag{20}$$

$$H' \;=\; \frac{L}{2\pi r^2\, k_{\mathrm{b}}} \;, \tag{21}$$

$$L' \;=\; \frac{1}{2\pi}\Big(p \,+\, 2\lambda H \,-\, 2k_{\mathrm{b}}\, H\big(H^2 - K\big) \,+\, \pi^{\alpha\beta}\, b_{\alpha\beta}\Big) \;, \tag{22}$$

$$\lambda' \;=\; \zeta \sin\varphi \left[\, \frac{2}{r}\, v' \;-\; \frac{\varphi' u}{\pi r^2} \,\right] \;, \tag{23}$$

$$u' \;=\; w \;, \tag{24}$$

and

$$w' \;=\; 2v' H \,+\, 2v H' \;, \tag{25}$$

where the $\pi^{\alpha\beta} b_{\alpha\beta}$ term in Eq. (22) is given by the second line of Eq. (15). We note that while the additional unknown $w$ is not required to pose the governing equations as a system of first-order ordinary differential equations, it is useful when solving the system of equations numerically, as will be discussed in subsequent sections.

## (b). Axial distance parametrization

While the area parametrization can describe axisymmetric surfaces of arbitrary geometry, it is also useful to consider an axisymmetric parametrization specialized to nearly cylindrical surfaces, given by

$$\boldsymbol{x}(\theta, z, t) \;=\; r(z,t)\, \boldsymbol{e}_r(\theta) \,+\, z\, \boldsymbol{e}_z \;, \tag{26}$$

where $\boldsymbol{e}_r$ and $\boldsymbol{e}_z$ are the usual orthonormal basis vectors in a cylindrical coordinate system. The surface parametrization in Eq. (26) is capable of describing nonlinear deformations that do not break a one-to-one mapping with the base cylindrical shape, and will be useful in subsequent analysis when we develop a weakly nonlinear model. Following the differential geometric surface description provided in Sec. I.1, we calculate the basis vectors as

$$\boldsymbol{a}_1 \;=\; r\, \boldsymbol{e}_\theta \;, \qquad \boldsymbol{a}_2 \;=\; r_{,z}\, \boldsymbol{e}_r \,+\, \boldsymbol{e}_z \;, \qquad \text{and} \qquad \boldsymbol{n} \;=\; (a_{22})^{-1/2}\big(\boldsymbol{e}_r \,-\, r_{,z}\, \boldsymbol{e}_z\big) \;, \tag{27}$$

where $a_{22} = \boldsymbol{a}_2 \cdot \boldsymbol{a}_2 = 1 + r_{,z}^2$ is the $(z, z)$ component of the metric tensor, and is introduced for notational convenience. The metric and curvature tensors are given by

$$a_{\alpha\beta} \;=\; \mathrm{diag}\big(r^2,\; 1 \,+\, r_{,z}^2\big) \qquad \text{and} \qquad b_{\alpha\beta} \;=\; (a_{22})^{-1/2}\, \mathrm{diag}\big(-r\,,\; r_{,zz}\big) \;. \tag{28}$$

Note the metric tensor can also be written as $\mathrm{diag}(a_{11}, a_{22})$. With the metric and curvature tensors, we calculate the mean and Gaussian curvatures to be respectively given by

$$H \;=\; \frac{-1}{2r\,(a_{22})^{1/2}}\,\Big(1 \,-\, (a_{22})^{-1}\, r_{,zz}\, r\Big) \qquad \text{and} \qquad K \;=\; \frac{-r_{,zz}}{r\,(a_{22})^2} \;. \tag{29}$$

Finally, the nonzero Christoffel symbols are given by

$$\Gamma^1_{12} = \Gamma^1_{21} = \frac{r_{,z}}{r} , \qquad \Gamma^2_{11} = -(a_{22})^{-1}\, r_{,z}\, r , \qquad \text{and} \qquad \Gamma^2_{22} = (a_{22})^{-1}\, r_{,z}\, r_{,zz} . \tag{30}$$

Substituting Eqs. (27)–(30) into the general governing equations (1)–(4), and after much algebra, we obtain the continuity, in-plane $z$, and shape equations respectively as

$$v^z_{,z} + v^z\, r_{,z}\left(\frac{1}{r} + \frac{r_{,zz}}{1+r^2_{,z}}\right) + \frac{r_{,t}}{r\big(1+r^2_{,z}\big)}\left(1 - \frac{r_{,zz}\, r}{1+r^2_{,z}}\right) = 0 , \tag{31}$$

$$\frac{2\zeta}{r}\left[\frac{r_{,t}\, r_{,z}\, r_{,zz}}{1+r^2_{,z}} - r_{,zz}\, v^z - r_{,zt}\right] + \big(1 + r^2_{,z}\big)\, \lambda_{,z} = 0 , \tag{32}$$

and

$$\begin{aligned} &p + 2\lambda H - 2k_{\mathrm{b}} H\big(H^2 - K\big) - \frac{k_{\mathrm{b}}}{r\,(1+r^2_{,z})^{1/2}} \cdot \frac{\partial}{\partial z}\left[\frac{r}{(1+r^2_{,z})^{1/2}}\, \frac{\partial H}{\partial z}\right] \\ &\quad - 2\zeta\left\{\frac{r_{,t}}{r^2(1+r^2_{,z})^{3/2}} + \frac{r_{,t}\, r_{,zz}}{r(1+r^2_{,z})^{5/2}} - \frac{v^z\, r_{,z}}{r^2(1+r^2_{,z})^{1/2}} + \frac{v^z\, r_{,z} r_{,zz}}{r(1+r^2_{,z})^{3/2}}\right\} = 0 . \end{aligned} \tag{33}$$

Equations (31)–(33) can also be found by starting with the general axisymmetric equations (13)–(15).

## 4. Linearized equations governing a lipid membrane tube

At this point, we simplify the general membrane equations to the case of small perturbations about an initially cylindrical membrane. As in Ref. [1], we first consider an unperturbed cylinder, and from the governing equations select a suitable base state. We then provide the linearized equations governing small perturbations to the base state, in both dimensional and dimensionless forms. While the previous section was concerned with only axisymmetric surfaces, here we consider both axisymmetric and non-axisymmetric perturbations.

### (a). Base state: Cylinder with constant axial velocity

We consider a perfectly cylindrical membrane tube of radius $r_0$, with position $\boldsymbol{x}_{(0)}(\theta, z) = r_0\, \boldsymbol{e}_r(\theta) + z\, \boldsymbol{e}_z$. Here, $\theta$ and $z$ are the polar angle and axial position of a cylindrical coordinate system, and a subscript or superscript '(0)' indicates the quantity refers to the unperturbed membrane. With the geometric description provided in Sec. I.1, we calculate

$$\begin{aligned} &\boldsymbol{a}^{(0)}_1 = r_0\, \boldsymbol{e}_\theta , \quad \boldsymbol{a}^{(0)}_2 = \boldsymbol{e}_z , \quad \boldsymbol{n}_{(0)} = \boldsymbol{e}_r , \quad a^{(0)}_{\alpha\beta} = \mathrm{diag}\,(r_0^2, 1) , \quad a^{\alpha\beta}_{(0)} = \mathrm{diag}\,(r_0^{-2}, 1) , \\ &b^{(0)}_{\alpha\beta} = \mathrm{diag}\,(-r_0, 0) , \qquad H_{(0)} = -1/(2r_0) , \qquad K_{(0)} = 0 , \qquad \text{and} \qquad \Gamma^{\alpha(0)}_{\lambda\mu} = 0 . \end{aligned} \tag{34}$$

The surface Laplacian of a scalar quantity is given by $\Delta_{\mathrm{s}}\,(\,\cdot\,) = r_0^{-2}(\,\cdot\,)_{,\theta\theta} + (\,\cdot\,)_{,zz}$. Since the tube is perfectly cylindrical, it has no velocity component in the normal direction, and the base membrane velocity is given by

$$\boldsymbol{v}_{(0)} = v^\alpha_{(0)} \boldsymbol{a}^{(0)}_\alpha = r_0\, v^\theta_{(0)} \boldsymbol{e}_\theta + v^z_{(0)} \boldsymbol{e}_z . \tag{35}$$

Note that $v^\theta_{(0)}$ has units of 1/time while $v^z_{(0)}$ has units of length/time, as per our differential geometric formulation. With Eqs. (34) and (35), the unperturbed continuity, in-plane $\theta$, in-plane $z$, and shape equations are found to be

$$v^\theta_{(0),\theta} + v^z_{(0),z} = 0 , \tag{36}$$

$$\frac{\zeta}{r_0}\Big(v^\theta_{(0),\theta\theta} + r_0^2\, v^\theta_{(0),zz}\Big) + \frac{1}{r_0}\, \lambda_{(0),\theta} = 0 , \tag{37}$$

$$\frac{\zeta}{r_0^2}\Big( v^z_{(0),\theta\theta} \,+\, r_0^2\, v^z_{(0),zz} \Big) \,+\, \lambda_{(0),z} \;=\; 0 \;, \tag{38}$$

and

$$p \,-\, \frac{\lambda_{(0)}}{r_0} \,+\, \frac{k_{\mathrm{b}}}{4r_0^3} \,+\, \frac{2\zeta}{r_0}\, v^z_{(0),z} \;=\; 0 \;. \tag{39}$$

By inspection, we find a valid solution to Eqs. (36)–(39) is given by

$$v^\theta_{(0)} \,=\, 0 \;, \qquad v^z_{(0)} \,=\, v_0 \;, \qquad v_{(0)} \,=\, 0 \;, \qquad \text{and} \qquad \lambda_{(0)} \,=\, \lambda_0 \,:=\, p r_0 \,+\, \frac{k_{\mathrm{b}}}{4r_0^2} \;, \tag{40}$$

where $p$, $v_0$, and $\lambda_0$ are all constants, and $v_0$ corresponds to the base velocity.

## (b). Perturbed equations and non-dimensionalization

We now perturb the base state, such that for a small parameter $\epsilon \ll 1$, the membrane position is given by $\boldsymbol{x}(\theta, z, t) = (r_0 + \epsilon\tilde{r}(\theta, z, t))\boldsymbol{e}_r(\theta) + z\boldsymbol{e}_z$. The fundamental unknowns are correspondingly expanded as

$$v^\theta \,=\, \epsilon\,\tilde{v}^\theta \;, \qquad v^z \,=\, v_0 \,+\, \epsilon\,\tilde{v}^z \;, \qquad v \,=\, \epsilon\,\tilde{r}_{,t} \;, \qquad \text{and} \qquad \lambda \,=\, \lambda_0 \,+\, \epsilon\,\tilde{\lambda} \;. \tag{41}$$

As detailed in the Supplemental Material (SM) of Ref. [1], the linearized first-order continuity, in-plane $\theta$, in-plane $z$, and shape equations are given by

$$r_0\,\tilde{v}^\theta_{,\theta} \,+\, r_0\,\tilde{v}^z_{,z} \,+\, \tilde{r}_{,t} \,+\, v_0\,\tilde{r}_{,z} \;=\; 0 \;, \tag{42}$$

$$\frac{\zeta}{r_0}\Big( \tilde{v}^\theta_{,\theta\theta} \,+\, r_0^2\,\tilde{v}^\theta_{,zz} \,+\, \frac{1}{r_0}\,\tilde{r}_{,t\theta} \,+\, \frac{v_0}{r_0}\,\tilde{r}_{,\theta z} \Big) \,+\, \frac{1}{r_0}\,\tilde{\lambda}_{,\theta} \;=\; 0 \;, \tag{43}$$

$$\frac{\zeta}{r_0^2}\Big( \tilde{v}^z_{,\theta\theta} \,+\, r_0^2\,\tilde{v}^z_{,zz} \,-\, r_0\,\tilde{r}_{,tz} \,-\, r_0 v_0\,\tilde{r}_{,zz} \Big) \,+\, \tilde{\lambda}_{,z} \;=\; 0 \;, \tag{44}$$

and

$$\frac{\lambda_0}{r_0^2}\Big(\tilde{r} \,+ r_0^2\,\Delta_{\mathrm{s}}\tilde{r}\Big) \,-\, \frac{\tilde{\lambda}}{r_0} - \frac{k_{\mathrm{b}}}{4r_0^4}\Big(3\tilde{r} \,+\, 4\tilde{r}_{,\theta\theta} \,+\, r_0^2\,\Delta_{\mathrm{s}}\,\tilde{r} \,+\, 2r_0^4\,\Delta_{\mathrm{s}}^2\,\tilde{r}\Big) \,+\, \frac{2\zeta}{r_0}\,\tilde{v}^z_{,z} \;=\; 0 \;. \tag{45}$$

At this point, we non-dimensionalize the perturbed equations (42)–(45). In our previous work [1], we used a scaling analysis to determine the magnitude of various unknown quantities, with different characteristic values depending on the system: for example, whether there was a base flow or whether the tube was thick or thin. In the present study, however, we seek a non-dimensionalization which is valid in all cases, such that by changing dimensionless parameters we can investigate the different regimes of cylindrical membrane dynamics. To this end, we define the timescale

$$\tau \,:=\, \frac{\zeta r_0^2}{k_{\mathrm{b}}} \tag{46}$$

and introduce the dimensionless quantities

$$\theta^* := \theta \;, \qquad z^* := \frac{z}{r_0} \;, \qquad \tilde{r}^* := \frac{\tilde{r}}{r_0} \;, \qquad \tilde{v}^{\theta *} := \tau\tilde{v}^\theta \;, \qquad \tilde{v}^{z*} := \frac{\tau\tilde{v}^z}{r_0} \;, \qquad \tilde{\lambda}^* := \frac{\tilde{\lambda}}{\lambda_0} \;, \qquad \text{and} \qquad t^* := \frac{t}{\tau} \;. \tag{47}$$

Importantly, Eq. (47) provides a scaling independent of the speed of the base flow: $\tilde{v}^{z*}$ is defined for both $v_0 = 0$ and $v_0 \neq 0$, unlike that of our previous analysis [1]. We next define the dimensionless Föppl–von Kármán number $\Gamma$ and Scriven–Love number $\mathit{SL}$ as

$$\Gamma \,=\, \frac{\lambda_0 r_0^2}{k_{\mathrm{b}}} \qquad \text{and} \qquad \mathit{SL} \,=\, \frac{\zeta v_0 r_0}{k_{\mathrm{b}}} \;, \tag{48}$$

as we introduced recently [1]. By substituting Eqs. (47) and (48) into Eqs. (42)–(45) and rearranging terms, we obtain the dimensionless perturbed governing equations as

$$\tilde{v}^{\theta *}_{,\theta^*} \,+\, \tilde{v}^{z*}_{,z^*} \,+\, \tilde{r}^*_{,t^*} \,+\, \mathit{SL}\,\tilde{r}^*_{,z^*} \;=\; 0 \;, \tag{49}$$

$$\tilde{v}^{\theta *}_{,\theta^*\theta^*} + \tilde{v}^{\theta *}_{,z^*z^*} + \tilde{r}^*_{,t^*\theta^*} + SL\,\tilde{r}^*_{,\theta^*z^*} + \Gamma\,\tilde{\lambda}^*_{,\theta} = 0\ , \tag{50}$$

$$\tilde{v}^{z *}_{,\theta^*\theta^*} + \tilde{v}^{z *}_{,z^*z^*} - \tilde{r}^*_{,t^*z^*} - SL\,\tilde{r}^*_{,z^*z^*} + \Gamma\,\tilde{\lambda}^*_{,z^*} = 0\ , \tag{51}$$

and

$$\Gamma\big(\tilde{r}^* + \Delta^*_{\mathrm{s}}\tilde{r}^* - \tilde{\lambda}^*\big) - \frac{1}{4}\big(3\tilde{r}^* + 4\tilde{r}^*_{,\theta^*\theta^*} + \Delta^*_{\mathrm{s}}\,\tilde{r}^* + 2\Delta^{*2}_{\mathrm{s}}\,\tilde{r}^*\big) + 2\tilde{v}^{z*}_{,z^*} = 0\ . \tag{52}$$

We reiterate here that the Föppl–von Kármán number is a measure of the relative importance of tension and bending forces, while the Scriven–Love number compares viscous to bending forces, all in the normal direction [1]. Importantly, given that our previous scaling analysis [1] revealed inertial effects to be negligible in the biological phenomena under investigation, the dynamics of lipid membrane tubes are completely specified by the values of $\Gamma$ and $SL$ *.

At this point, we find it useful to note that given our base solution (40), the unperturbed shape equation (39) can be written in dimensionless form as

$$\Gamma = \frac{p\,r_0^3}{k_{\mathrm{b}}} + \frac{1}{4}\ . \tag{53}$$

Thus, for a tube with a given bending modulus $k_{\mathrm{b}}$ and initial radius $r_0$, the jump in the normal stress $p$ determines the value of $\Gamma$. We define the value

$$\Gamma_0 := \frac{1}{4} \tag{54}$$

to be the Föppl–von Kármán number when $p = 0$, such that when $\Gamma > \Gamma_0$ the surrounding fluid inflates the tube while if $\Gamma < \Gamma_0$ the surrounding fluid compresses the tube. In the present work, we are concerned only with the former case, and leave the investigation of tubes under compression to a future study.

## (c). Axisymmetric evolution equation

We previously mentioned that axisymmetric lipid membrane tubes will be particularly relevant in our later investigations. In the case where the tube is axisymmetric, such that $\tilde{v}^\theta = 0$ and no quantities depend on $\theta$, the four governing equations (49)–(52) can be condensed into a single equation for the perturbed membrane shape, $\tilde{r}$. To this end, we first integrate Eq.(51) with respect to $z^*$, thereby obtaining

$$-\,\tilde{r}^*_{,t^*} - SL\,\tilde{r}^*_{,z^*} + \tilde{v}^{z*}_{,z^*} + \Gamma\,\tilde{\lambda}^* = 0\ , \tag{55}$$

where we set the integration constant to zero such that an unperturbed cylinder ($\tilde{r}^* = 0$) has a constant, unperturbed tension ($\tilde{\lambda}^* = 0$). Next, we substitute Eq. (55) into the linearized shape equation (52) and obtain

$$-\,3\big(\tilde{r}^*_{,t^*} + SL\,\tilde{r}^*_{,z^*}\big) + \tilde{v}^{z*}_{,z^*} + \big(\Gamma - \Gamma_{\mathrm{c}}\big)\tilde{r}^* + \big(\Gamma - \Gamma_0\big)\tilde{r}^*_{,z^*z^*} - \frac{1}{2}\,\tilde{r}_{,z^*z^*z^*z^*} = 0\ . \tag{56}$$

Moreover, we notice from the continuity equation (49) that

$$\tilde{v}^{z*}_{,z^*} = -\tilde{r}^*_{,t^*} - SL\,\tilde{r}^*_{,z^*}\ , \tag{57}$$

and substitute this expression of the axial velocity gradient into Eq. (56). We thus obtain the following evolution equation, involving only the shape perturbation, presented as Eq. 1 in the main text:

$$\tilde{r}^*_{,t^*} + SL\,\tilde{r}^*_{,z^*} = \left(\frac{\Gamma - \Gamma_{\mathrm{c}}}{4}\right)\tilde{r}^* + \left(\frac{\Gamma - \Gamma_0}{4}\right)\tilde{r}^*_{,z^*z^*} - \frac{1}{8}\,\tilde{r}^*_{,z^*z^*z^*z^*}\ . \tag{58}$$

*When the dynamics of the surrounding fluid are considered, the governing equations also depend on the Boussinesq number—defined as $Bo = \zeta/(r_0\mu)$, where $\mu$ is the fluid shear viscosity [8].

## II. Temporal stability analysis

In this section, we follow standard techniques [9] to analyze the stability of lipid membrane tubes in response to global shape perturbations. We begin by decomposing all fundamental unknowns into normal modes, and then obtain the algebraic equations governing the normal mode coefficients. We next calculate the dispersion relation, and end by providing stability criteria. Note that from now on, all calculations are in terms of dimensionless quantities, and we drop the '$*$' superscript for notational convenience.

### 1. Decomposition into normal modes

The perturbed governing equations (49)–(52) contain four fundamental unknowns, namely the dimensionless perturbed quantities $\tilde{r}$, $\tilde{v}^\theta$, $\tilde{v}^z$, and $\tilde{\lambda}$. We use the shorthand $\tilde{A}$ to denote any of these four unknowns, which are decomposed into normal modes according to

$$\tilde{A}(\theta, z, t) \,=\, \sum_{m,q} \hat{A}_{m,q} \, \exp\big[\mathrm{i}\big(m\theta + qz - \omega t\big)\big] \; . \tag{59}$$

In Eq. (59), the angular wavenumber $m \in \mathbb{Z}$, the dimensionless axial wavenumber $q \in \mathbb{R}$, and the dimensionless frequency $\omega = \omega^{(r)} + \mathrm{i}\omega^{(i)} \in \mathbb{C}$; here $q$ is scaled by $1/r_0$ and $\omega$ is scaled by $1/\tau$ (46). For quantities with the functional dependence given in Eq. (59),

$$\partial_\theta \,=\, \mathrm{i}m \;, \quad \partial_z \,=\, \mathrm{i}q \;, \quad \partial_t \,=\, -\mathrm{i}\omega \;, \quad \partial^2_\theta \,=\, -m^2 \;, \quad \partial^2_z \,=\, -q^2 \;, \quad \text{and} \quad \Delta_{\mathrm{s}} \,=\, -(m^2 + q^2) \; . \tag{60}$$

Substituting Eqs. (59) and (60) into Eqs. (49)–(52) and recognizing all normal modes are independent, we obtain the equations governing the normal mode coefficients as

$$m\hat{v}^\theta \,+\, q\hat{v}^z \,+\, \big(\mathit{SL}\,q \,-\, \omega\big)\hat{r} \,=\, 0 \; , \tag{61}$$

$$-\big(m^2 \,+\, q^2\big)\hat{v}^\theta \,+\, \big(\omega m \,-\, \mathit{SL}\,qm\big)\hat{r} \,+\, \mathrm{i}m\Gamma\,\hat{\lambda} \,=\, 0 \; , \tag{62}$$

$$-\big(m^2 \,+\, q^2\big)\hat{v}^z \,+\, \big(\mathit{SL}\,q^2 \,-\, \omega q\big)\hat{r} \,+\, \mathrm{i}q\Gamma\,\hat{\lambda} \,=\, 0 \; , \tag{63}$$

and

$$\Big\{\Gamma\big(1 \,-\, m^2 \,-\, q^2\big) \,-\, \frac{1}{4}\Big[3 \,-\, 5m^2 \,-\, q^2 \,+\, 2\big(m^2 \,+\, q^2\big)^2\Big]\Big\}\,\hat{r} \,-\, \Gamma\hat{\lambda} \,+\, 2\mathrm{i}q\,\hat{v}^z \,=\, 0 \; . \tag{64}$$

### 2. Dispersion relation

The system of Eqs. (61)–(64) consists of four linear, algebraic equations in the four unknowns $\hat{r}$, $\hat{v}^\theta$, $\hat{v}^z$, and $\hat{\lambda}$. Various techniques can be used to calculate the dispersion relation $\omega = \omega(q)$; in what follows, we use a series of algebraic manipulations. Recognizing the in-plane $z$-equation (63) and the shape equation (64) do not involve $\hat{v}^\theta$, we first seek to combine Eqs. (61) and (62) to eliminate $\hat{v}^\theta$. To this end, we multiply the continuity equation (61) by $(m^2 + q^2)$, multiply the in-plane $\theta$ equation by $m$, and add the two to obtain

$$-\,q^2\big(\omega \,-\, \mathit{SL}\,q\big)\hat{r} \,+\, q\big(m^2 \,+\, q^2\big)\hat{v}^z \,+\, \mathrm{i}\Gamma m^2\,\hat{\lambda} \,=\, 0 \; . \tag{65}$$

We next seek to remove the $\hat{v}^z$ dependence from the system of equations. By multiplying the shape equation (64) by $(m^2 + q^2)$, multiplying Eq. (65) by $-2\mathrm{i}$, and combining the results, we find

$$\big[\alpha\big(m^2 \,+\, q^2\big) \,+\, 2\mathrm{i}q^2\big(\omega \,-\, \mathit{SL}\,q\big)\big]\hat{r} \,+\, \Gamma\big(m^2 \,-\, q^2\big)\hat{\lambda} \,=\, 0 \; , \tag{66}$$

where $\alpha$ is a shorthand for the prefactor coefficient of $\hat{r}$ in Eq. (64). Similarly, multiplying the in-plane $z$-equation (63) by $q$ and adding Eq. (65) yields

$$-\,2q^2\big(\omega \,-\, \mathit{SL}\,q\big)\hat{r} \,+\, \mathrm{i}\Gamma\big(m^2 \,+\, q^2\big)\hat{\lambda} \,=\, 0 \; . \tag{67}$$

With Eqs. (66) and (67), we simplified our initial set of equations into a system with two equations and two unknowns.

Finally, we combine Eqs. (66) and (67) to obtain an equation for $\hat{r}$. By multiplying Eq. (66) by $\mathrm{i}(m^2+q^2)$, multiplying Eq. (67) by $(q^2 - m^2)$, and summing the two results, we obtain

$$\Big[\alpha\mathrm{i}\big(m^2 + q^2\big)^2 - 4q^4\big(\omega - \mathit{SL}\,q\big)\Big]\hat{r} = 0 \,. \tag{68}$$

To obtain a nontrivial solution, i.e. one for which $\hat{r} \neq 0$, we require

$$\alpha\mathrm{i}\big(m^2 + q^2\big)^2 - 4q^4\big(\omega - \mathit{SL}\,q\big) = 0 \,. \tag{69}$$

Solving Eq. (69) for $\omega$ and inserting the expression for $\alpha$ yields the dispersion relation

$$\omega = \mathit{SL}\,q + \mathrm{i}\,\frac{(m^2 + q^2)^2}{4q^4}\left\{\Gamma\big(1 - m^2 - q^2\big) - \frac{1}{4}\Big[3 - 5m^2 - q^2 + 2\big(m^2 + q^2\big)^2\Big]\right\} . \tag{70}$$

Given the form of our decomposition into normal modes (59), Eq. (70) indicates that a base flow ($\mathit{SL} \neq 0$) leads to temporally oscillating solutions, while the base tension (captured by $\Gamma$) dictates the growth rate of the perturbation envelope. Importantly, our choice of non-dimensionalization (47, 48) allows for the two dimensionless numbers $\mathit{SL}$ and $\Gamma$ to be decoupled in the dispersion relation (70).

## 3. Linear stability analysis

With the decomposition into normal modes given in Eq. (41), our system is unstable when $\omega^{(i)} > 0$. For the calculated dispersion relation (70), a lipid membrane tube is unstable when

$$\Gamma\big(1 - m^2 - q^2\big) - \frac{1}{4}\Big[3 - 5m^2 - q^2 + 2\big(m^2 + q^2\big)^2\Big] > 0 \,. \tag{71}$$

As the angular wavenumber $m \in \mathbb{Z}$ is discrete, for each value of $m$ we use Eq. (71) to determine which points in the $(\Gamma, q)$ plane are unstable. The unstable regions for $m = 0$, $m = 1$, and $m = 2$ are plotted in Fig. 2. As first pointed out in Ref. [8], the amplitude of modes with $m \geq 1$ can only grow in time when the tube is under compression, for which $\Gamma < \Gamma_0$. Additionally, for tubes under tension, only axisymmetric $m = 0$ modes are unstable. As the present study is only concerned with tubes under tension, only axisymmetric perturbations are considered from this point onwards.

When $m = 0$, the dispersion relation (70) simplifies to

$$\omega = \mathit{SL}\,q + \frac{\mathrm{i}}{4}\left\{\Gamma\big(1 - q^2\big) - \frac{1}{4}\Big[3 - q^2 + 2q^4\Big]\right\} , \tag{72}$$

written as Eq. (3) in the main text. Moreover, the instability criterion (71) simplifies to

$$\Gamma\big(1 - q^2\big) - \frac{1}{4}\Big[3 - q^2 + 2q^4\Big] > 0 \,. \tag{73}$$

Note that Eqs. (72) and (73) can also be obtained directly by substituting the normal mode decomposition for $\tilde{r}$ (59) into Eq. (58). The real and imaginary parts of the axisymmetric dispersion relation (72) are plotted in Fig. 3, from which we make several additional observations. First, as found in Refs. [8, 10–12] and confirmed by Fig. 2, a necessary condition for a membrane tube to be unstable is

$$\Gamma > \Gamma_{\mathrm{c}} \,, \qquad \text{where} \qquad \Gamma_{\mathrm{c}} := \frac{3}{4} \tag{74}$$

is the critical value of the Föppl–von Kármán number at which a lipid membrane tube first becomes unstable. Second, given a membrane tube with $\Gamma > \Gamma_{\mathrm{c}}$, $q = 0$ is the fastest growing mode, for which the corresponding growth rate $\omega^{(i)}_{\mathrm{max}}$ is given by

$$\omega^{(i)}_{\mathrm{max}} = \frac{\Gamma - \Gamma_{\mathrm{c}}}{4} \,. \tag{75}$$

Note that in contrast, past studies which accounted for the dynamics of the surrounding fluid—which are neglected in the present work—found a nonzero, finite wavenumber to have the maximum growth rate when

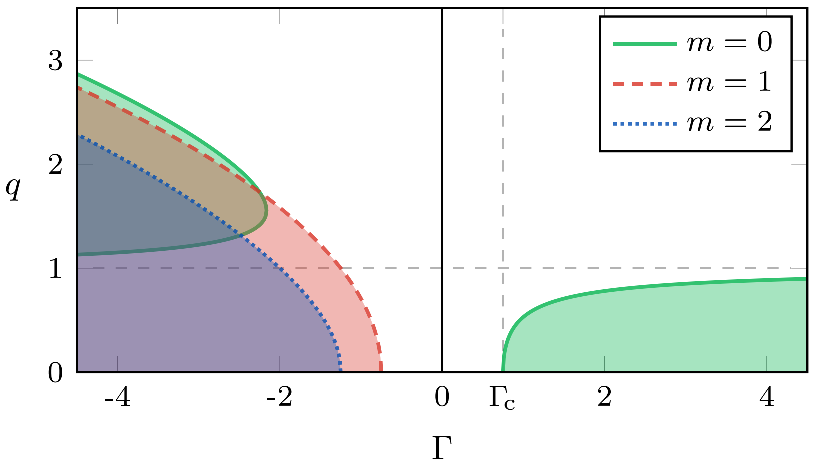


Figure 2: Stable and unstable regimes for angular wavenumbers $m = 0$ (green, solid), $m = 1$ (red, dashed), and $m = 2$ (blue, dotted), with the unstable regimes being shaded. Only long wavelength axisymmetric $m = 0$ modes are unstable when $\Gamma > \Gamma_0 = {}^1\!/_4$, with the solid green line being the marginally stable wavenumber $q_{ms}$ calculated in Eq. (76). Short wavelength axisymmetric modes are also unstable when the tube is under compression, and $\Gamma < \Gamma_0$. Non-axisymmetric modes are only unstable when the tube is under compression.

the tube is unstable [8, 12]. We find that when $\Gamma > \Gamma_c$, unstable perturbations are limited to a finite range of wavenumbers $q \in [0, q_{ms}]$, where $q_{ms}$ is the marginally stable wavenumber for which $\omega^{(i)} = 0$. Applying this definition of $q_{ms}$ to Eq. (72), we obtain

$$q_{ms} = \sqrt{-(\Gamma - \Gamma_0) + \sqrt{(\Gamma - \Gamma_0)^2 + 2(\Gamma - \Gamma_c)}} = \sqrt{-\Gamma + \frac{1}{4} + \sqrt{\Gamma^2 + \frac{3}{2}\Gamma - \frac{23}{16}}}\ , \tag{76}$$

in agreement with Ref. [12]. The marginally stable wavenumber $q_{ms}$ for axisymmetric $m = 0$ modes is plotted as the solid green line in Fig. 2 when $\Gamma > \Gamma_0$, and also predicts the point where $\omega^{(i)}$ crosses zero in Fig. 3a. Moreover, in the limit of $\Gamma \to \Gamma_c^+$, we find $q_{ms} \sim (\Gamma - \Gamma_c)^{1/2} \to 0$ such that only infinitely long axial perturbations are unstable. Finally, we observe that the Scriven–Love number *SL* does not affect the growth rate of the perturbed system, but rather provides an oscillation frequency to the temporal evolution of axisymmetric modes (see Fig. 3b).

# III. Spatiotemporal stability analysis

In the analysis presented thus far, we proposed that the wavenumber $q \in \mathbb{R}$, while the frequency $\omega \in \mathbb{C}$. In doing so, we restricted the spatial behavior of perturbations to a superposition of global sinusoidal modes and investigated how such disturbances evolved in time. Such a framework is only appropriate for a *temporal* stability analysis. However, in the case of a tube with nonzero base flow, sinusoidal modes display time periodicity and the tube also possesses a preferred directionality—which can bias the spatial evolution of perturbations, particularly if they are initially localized in space. Indeed, when local drug treatments were administered to *in vitro* cultures of axons, propagating fronts ensued from the neuronal growth cone to the cell body in the direction of lipid flow [13]. Various studies on other physical systems such as plasmas [14–16], geophysical flows [17, 18], open fluid flows such as wakes, jets and boundary layers [19, 20], cylindrical fluid columns [21], and more recently thin films on substrates [22, 23], have shown the presence of a base flow is best understood by addressing the following question: How does the unstable system respond to an initially local, rather than global, perturbation? We now address this question by extending the techniques presented thus far to perform a *spatiotemporal* stability analysis.

In this section, we follow procedures developed in [19, 20, 24] to investigate how a membrane tube with a non-zero base flow responds to an initially localized shape perturbation. To this end, we hereafter consider

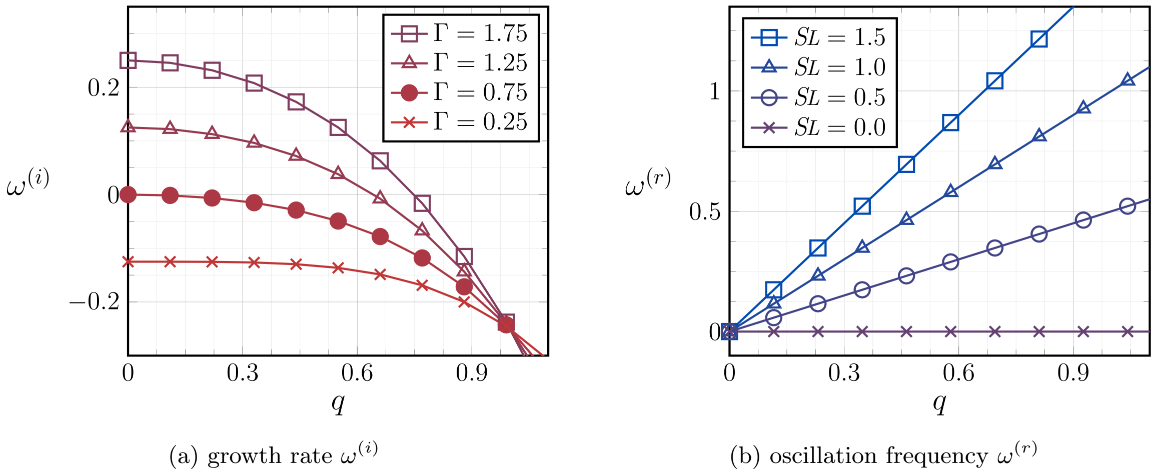


Figure 3: Plots of (a) the growth rate $\omega^{(i)}$ and (b) the oscillation frequency $\omega^{(r)}$ of a perturbed axisymmetric membrane tube, for different values of the Föppl–von Kármán number $\Gamma$ and the Scriven–Love number *SL*. Note that the growth rate only depends on $\Gamma$, while the oscillation frequency only depends on *SL*. (a) The growth rate is negative and the tube is stable when $\Gamma < \Gamma_c = {}^3\!/\!_4$. When $\Gamma > \Gamma_c$, the growth rate is positive for modes $q \in (0, q_{ms})$, with the marginally stable wavenumber calculated in Eq. (76). For unstable tubes, $q = 0$ is the fastest growing mode. (b) The oscillation frequency is linear in the wavenumber, with the proportionality constant being the Scriven–Love number *SL*.

complex wavenumbers $q = q^{(r)} + \mathrm{i}q^{(i)} \in \mathbb{C}$ and frequencies $\omega = \omega^{(r)} + \mathrm{i}\omega^{(i)} \in \mathbb{C}$, such that an initially localized perturbation can be studied via the normal mode decomposition in Eq. (59) [25]. As mentioned previously, the Föppl–von Kármán number alone dictates whether perturbations are amplified or not. However, the base flow speed, as captured in the Scriven–Love number, determines how initially localized perturbations spatially invade the tube over time. For a fixed observer at a local station along the tube, the fate of the observed local disturbances will depend on the competition between the amplification of the instability, characterized by $\Gamma$, and its advection downstream, captured by *SL*: for larger values of the Scriven–Love number, growing perturbations are more quickly advected downstream. Eventually, the instability is advected faster down the tube than it grows, and the instability undergoes a so-called *absolute-to-convective* transition. In the case of an *absolutely unstable* system, the initially localized perturbation will eventually invade the entire domain. In contrast, for a *convectively unstable* system, any stationary observer will eventually see an unperturbed tube—despite the perturbation continuing to grow in time. For the remainder of this section, we use a spatiotemporal stability analysis to determine under what conditions a lipid membrane tube is absolutely or convectively unstable, with our main results presented in Figs. 1(a) and 2 of the main text.

## 1. Saddle points of the dispersion relation

We begin by considering a local perturbation to an unstable lipid membrane tube, for which $\Gamma > \Gamma_c$. As the perturbation grows, at long times a stationary observer will, by definition, see disturbances of zero group velocity. The so-called 'absolute wavenumber' $q_0$ and 'absolute frequency' $\omega_0$ corresponding to zero group velocity disturbances are determined according to

$$\left.\frac{\mathrm{d}\omega}{\mathrm{d}q}\right|_{q_0} = 0 \qquad \text{and} \qquad \omega_0 = \omega(q_0)\ , \tag{77}$$

where it is important to reiterate that here and henceforth, $\omega$ and $q$ are complex variables. As discussed in Ref. [20], the pair $(q_0, \omega_0)$ is often called a saddle point, due to the nature of $\omega^{(r)}$ when plotted as a function of $q^{(r)}$ and $q^{(i)}$. We accordingly refer to $(q_0, \omega_0)$ as a saddle point for the remainder of our analysis.

By applying the two saddle point criteria (77) to the dispersion relation (72), we respectively obtain the conditions

$$SL - \frac{\mathrm{i}}{2}\left\{\left(\Gamma - \Gamma_0\right) q_0 + q_0^3\right\} = 0 \tag{78}$$

and

$$\omega_0 = SL\, q_0 + \frac{\mathrm{i}}{8}\left\{2\left(\Gamma - \Gamma_\mathrm{c}\right) - 2\left(\Gamma - \Gamma_0\right) q_0^2 - q_0^4\right\} . \tag{79}$$

Next, the relations $q_0 = q_0^{(r)} + \mathrm{i} q_0^{(i)}$ and $\omega_0 = \omega_0^{(r)} + \mathrm{i}\omega_0^{(i)}$ are substituted into Eqs. (78) and (79), and the resulting equations are split into real and imaginary components to yield four conditions, respectively given by

$$2\,SL + \left(\Gamma - \Gamma_0\right) q_0^{(i)} + 3\left(q_0^{(r)}\right)^2 q_0^{(i)} - \left(q_0^{(i)}\right)^3 = 0 , \tag{80}$$

$$q_0^{(r)}\left[\left(\Gamma - \Gamma_0\right) + \left(q_0^{(r)}\right)^2 - 3\left(q_0^{(i)}\right)^2\right] = 0 , \tag{81}$$

$$\omega_0^{(r)} = q_0^{(r)}\left\{SL + \frac{1}{2} q_0^{(i)}\left[\left(\Gamma - \Gamma_0\right) + \left(q_0^{(r)}\right)^2 - \left(q_0^{(i)}\right)^2\right]\right\} , \tag{82}$$

and

$$\omega_0^{(i)} = SL\, q_0^{(i)} + \frac{1}{8}\left\{2\left(\Gamma - \Gamma_\mathrm{c}\right) + 2\left(\Gamma - \Gamma_0\right)\left[\left(q_0^{(i)}\right)^2 - \left(q_0^{(r)}\right)^2\right] - \left(q_0^{(r)}\right)^4 + 6\left(q_0^{(r)}\right)^2\left(q_0^{(i)}\right)^2 - \left(q_0^{(i)}\right)^4\right\} . \tag{83}$$

We now have four equations (80–83) corresponding to the four unknowns $q_0^{(r)}$, $q_0^{(i)}$, $\omega_0^{(r)}$, and $\omega_0^{(i)}$, for any values of the parameters $SL$ and $\Gamma$.

At this point, we seek the boundary between absolutely and convectively unstable regimes. We recognize that a stationary observer will see a positive growth rate, for which $\omega_0^{(i)} > 0$, when the tube is absolutely unstable, and a negative growth rate, with $\omega_0^{(i)} < 0$, when the tube is convectively unstable. A necessary condition for the absolute-to-convective transition is thus given by

$$\omega_0^{(i)} = 0 . \tag{84}$$

With Eq. (84), we now have an additional equation relating $SL$ and $\Gamma$. In what follows, for every unstable tube with $\Gamma > \Gamma_\mathrm{c}$ we calculate the saddle point $(q_0, \omega_0)$ and the critical Scriven–Love number $SL_\mathrm{ac}(\Gamma)$ corresponding to the absolute-to-convective transition, for which Eqs. (80)–(84) are satisfied. Due to Eq. (81), this calculation is split into two cases, as either

$$q_0^{(r)} = 0 \qquad \text{or} \qquad \left(q_0^{(r)}\right)^2 = 3\left(q_0^{(i)}\right)^2 - \left(\Gamma - \Gamma_0\right) . \tag{85}$$

We note that Eq. (84) is a necessary but not sufficient condition for the absolute-to-convective transition—implying our calculation of the saddle point and critical base flow velocity may not be physical, as established in previous works [14, 15, 19, 26]. Consequently, in Sec. III.2 we investigate whether the calculated values of $q_0$, $\omega_0$, and $SL_\mathrm{ac}$ are physical or spurious.

### (a). Purely imaginary absolute wavenumber

When $q_0^{(r)} = 0$, Eqs. (80)–(84) simplify to

$$2\,SL_\mathrm{ac} + \left(\Gamma - \Gamma_0\right) q_0^{(i)} - \left(q_0^{(i)}\right)^3 = 0 , \tag{86}$$

$$SL_\mathrm{ac}\, q_0^{(i)} + \frac{1}{8}\left\{2\left(\Gamma - \Gamma_\mathrm{c}\right) + 2\left(\Gamma - \Gamma_0\right)\left(q_0^{(i)}\right)^2 - \left(q_0^{(i)}\right)^4\right\} = 0 , \tag{87}$$

and

$$\omega_0^{(r)} = 0 . \tag{88}$$

If $q_0^{(i)} = 0$ as well, Eqs. (86) and (87) reduce to $\Gamma = \Gamma_c$ and $SL_{ac} = 0$. Since we are interested in obtaining $SL_{ac}$ for all $\Gamma$, we assume $q_0^{(i)} \neq 0$. This allows us to multiply Eq. (86) by $-q_0^{(i)}$ and add the result to twice Eq. (87), which after some rearrangement yields the following equation for $q_0^{(i)}$:

$$3\big(q_0^{(i)}\big)^4 \;-\; 2\big(\Gamma-\Gamma_0\big)\big(q_0^{(i)}\big)^2 \;+\; 2\big(\Gamma-\Gamma_c\big) \;=\; 0\;. \tag{89}$$

As $q_0^{(i)} \in \mathbb{R}$, we find Eq. (89) has only real roots when

$$\Gamma \in \Omega_A := [\Gamma_c, \Gamma_1] \cup [\Gamma_2, \infty)\;, \tag{90}$$

where $\Gamma_1$ and $\Gamma_2$ are defined as

$$\Gamma_1 := \frac{13}{4} - \sqrt{6} \approx 0.801 \qquad \text{and} \qquad \Gamma_2 := \frac{13}{4} + \sqrt{6} \approx 5.699\;. \tag{91}$$

Thus, the four solutions of Eq. (89) for $q_0^{(i)}$ are given by

$$q_0^{(i)} \;=\; \pm\frac{1}{\sqrt{3}}\sqrt{\big(\Gamma-\Gamma_0\big) \pm \sqrt{\big(\Gamma-\Gamma_0\big)^2 \;-\; 6\big(\Gamma-\Gamma_c\big)}}\;, \qquad \text{with} \qquad \Gamma\in\Omega_A\;. \tag{92}$$

At this point, we note that of the four solutions in Eq. (92), two are positive and two are negative. However, our spatial ansatz $\sim \exp(\mathrm{i}qz) = \exp(-q^{(i)}z)\exp(\mathrm{i}q^{(r)}z)$ and the base flow is in the positive $z$-direction. As we are interested in the absolute-to-convective transition, for which a perturbation initially at the origin ($z = 0$) grows downstream ($z > 0$), we choose only the negative solutions of $q_0^{(i)}$ in Eq. (92) such that our spatial ansatz grows downstream, and find

$$\begin{aligned} q_0^{(i)\pm} \;&=\; \frac{-1}{\sqrt{3}}\sqrt{\big(\Gamma-\Gamma_0\big) \pm \sqrt{\big(\Gamma-\Gamma_0\big)^2 \;-\; 6\big(\Gamma-\Gamma_c\big)}} \\ &=\; \frac{-1}{2\sqrt{3}}\sqrt{4\Gamma - 1 \pm \sqrt{16\Gamma^2 \;-\; 104\Gamma \;+\; 73}}\;, \qquad\qquad \text{with} \qquad \Gamma\in\Omega_A\;. \end{aligned} \tag{93}$$

Substituting Eq. (93) into Eq. (86) yields two solutions for $SL_{ac}$ as

$$SL_{ac}^{\pm} \;=\; \frac{-1}{48\sqrt{3}}\sqrt{4\Gamma-1 \pm \sqrt{16\Gamma^2 - 104\Gamma + 73}}\,\Big(-8\Gamma + 2 \pm \sqrt{16\Gamma^2 - 104\Gamma + 73}\Big)\;, \tag{94}$$

with $\Gamma \in \Omega_A$. However, we will show subsequently that only one of these absolute-to-convective Scriven–Love numbers, namely $SL_{ac}^{-}$, is physically meaningful. Before doing so, we next consider the other possible case from Eq. (85), where $q_0^{(r)} \neq 0$.

### (b). Absolute wavenumber with nonzero real and imaginary parts

When $q_0^{(r)} \neq 0$, Eq. (81) requires the real and imaginary parts of the absolute wavenumber to be related by [see also Eq. $(85)_2$]

$$\big(q_0^{(r)}\big)^2 \;=\; 3\big(q_0^{(i)}\big)^2 \;-\; \big(\Gamma-\Gamma_0\big)\;. \tag{95}$$

By substituting Eq. (95) into Eqs. (80) and (83), making use of Eq. (84), and rearranging terms, we obtain two equations for $q_0^{(i)}(\Gamma)$ and $SL_{ac}(\Gamma)$—given by

$$SL_{ac} \;+\; q_0^{(i)}\big[\,4\big(q_0^{(i)}\big)^2 \;-\; \big(\Gamma-\Gamma_0\big)\big] \;=\; 0 \tag{96}$$

and

$$SL_{ac}\,q_0^{(i)} \;+\; \big(q_0^{(i)}\big)^4 \;-\; \frac{\Gamma-\Gamma_0}{2}\,\big(q_0^{(i)}\big)^2 \;+\; \frac{1}{8}\,\big(\Gamma-\Gamma_0\big)^2 \;+\; \frac{1}{4}\,\big(\Gamma-\Gamma_c\big) \;=\; 0\;. \tag{97}$$

If we assume $q_0^{(i)} = 0$, then Eqs. (96) and (97) require $SL_{\rm ac} = 0$ and $\Gamma < \Gamma_{\rm c}$: an unphysical result, since the absolute-to-convective transition is only physically meaningful for unstable tubes, in which $\Gamma > \Gamma_{\rm c}$. Thus $q_0^{(i)} \neq 0$, allowing us to multiply Eq. (96) by $-q_0^{(i)}$ and add the result to Eq. (97) to obtain

$$24\big(q_0^{(i)}\big)^4 - 4\big(\Gamma - \Gamma_0\big)\big(q_0^{(i)}\big)^2 - \big(\Gamma - \Gamma_0\big)^2 - 2\big(\Gamma - \Gamma_{\rm c}\big) = 0 \,. \tag{98}$$

Solving Eq. (98) for $q_0^{(i)}$, with the requirements that (i) $q_0^{(i)} \in \mathbb{R}$ and (ii) $q_0^{(i)} < 0$ such that the mode grows spatially downstream ($z > 0$), we find

$$q_0^{(i)} = -\frac{1}{4\sqrt{3}} \sqrt{4\Gamma - 1 + \sqrt{112\Gamma^2 + 136\Gamma - 137}} \;, \tag{99}$$

for all $\Gamma > \Gamma_{\rm c}$. By substituting Eq. (99) into Eq. (95), we obtain the real part of the absolute wavenumber as

$$q_0^{(r)\pm} = \pm\frac{1}{4} \sqrt{-12\Gamma + 3 + \sqrt{112\Gamma^2 + 136\Gamma - 137}} \;. \tag{100}$$

However, as $q_0^{(r)} \in \mathbb{R}$, Eq. (100) is only meaningful when $-12\Gamma + 3 + \sqrt{112\Gamma^2 + 136\Gamma - 137} > 0$, which requires

$$\Gamma \in \Omega_{\rm B} := (\Gamma_1, \Gamma_2) \;, \tag{101}$$

where $\Gamma_1$ and $\Gamma_2$ were defined in Eq. (91). Interestingly, $\Omega_{\rm B}$ is complementary to $\Omega_{\rm A}$, such that $\Omega_{\rm A} \cap \Omega_{\rm B} = \varnothing$ and $\Omega_{\rm A} \cup \Omega_{\rm B} = [\Gamma_{\rm c}, \infty)$, the latter being the entire range of Föppl–von Kármán numbers corresponding to unstable tubes. For $\Gamma \in \Omega_{\rm B}$, we determine the absolute-to-convective Scriven–Love number $SL_{\rm ac}^-$ via Eq. (96) as

$$SL_{\rm ac}^- = \frac{1}{48\sqrt{3}} \sqrt{4\Gamma - 1 + \sqrt{112\Gamma^2 + 136\Gamma - 137}} \Big( -8\Gamma + 2 + \sqrt{112\Gamma^2 + 136\Gamma - 137} \Big) \,. \tag{102}$$

Note that when $\Gamma \in \Omega_{\rm B}$, there is only a single value of $SL_{\rm ac}$ (102), while for $\Gamma \in \Omega_{\rm A}$ we obtained two values of $SL_{\rm ac}$ (94). Finally, we calculate the real part of the absolute frequency, $\omega_0^{(r)}$, using Eq. (82), and find

$$\begin{aligned} \omega_0^{(r)\pm} = \mp\frac{1}{128\sqrt{3}} \sqrt{16\Gamma^2 + 40\Gamma - 35 - \tfrac{1}{2}\big(4\Gamma - 1\big)\sqrt{112\Gamma^2 + 136\Gamma - 137}} \times \dots \\ \dots \times \Big(12\Gamma - 3 - \sqrt{112\Gamma^2 + 136\Gamma - 137}\Big) \,. \end{aligned} \tag{103}$$

## 2. Absolute to convective transition

At this point, we found analytical expressions for the saddle point $(q_0, \omega_0)$ and the absolute-to-convective Scriven–Love number $SL_{\rm ac}$ by solving the saddle point and growth rate conditions in Eqs. (80)–(84) simultaneously; all quantities have different expressions depending on whether $\Gamma \in \Omega_{\rm A}$ or $\Gamma \in \Omega_{\rm B}$. However, as mentioned earlier, the condition $\omega_0^{(i)} = 0$ (84) is necessary but not sufficient to determine $SL_{\rm ac}$ [14, 15, 20]. In this section, we evaluate whether the previously calculated values of $SL_{\rm ac}$ do in fact describe where our cylindrical membrane system transitions from being absolutely unstable to being convectively unstable. We follow the approach detailed by Bers and Briggs [14] and subsequently other authors [19, 26], in which a geometric criterion was found to determine if a saddle point is associated with a transition from an absolute to a convective instability. A rigorous explanation of this criterion is outside the scope of our work, and requires long-time asymptotics and an analysis of pole singularities in the complex plane (see, for example, Ref. [20]). However, in what follows, we describe several major themes of the criterion and then provide the procedure used to determine if the saddle points are physical or spurious in nature. The description is drawn almost entirely from the analysis by P. Huerre and M. Rossi [20, Sec. 3], who analyze the absolute-to-convective transition of the well-known Ginzburg–Landau (GL) equation. We highly recommend Ref. [20] to interested readers, and as a result highlight its relevant sections in the following presentation.

The geometric criterion obtained by Bers and Briggs [14] is largely concerned with the nature of solutions to the dispersion relation $\omega = \omega(q)$ in the vicinity of the saddle point. By Taylor expanding the dispersion relation about the saddle point and recalling $\omega'(q_0) = 0$ from Eq. $(77)_1$, one obtains

$$\omega - \omega_0 \approx \frac{\omega''(q_0)}{2}(q - q_0)^2 , \qquad \text{or equivalently} \qquad q - q_0 \approx \pm\left(\frac{2}{\omega''(q_0)}\right)^{1/2}(\omega - \omega_0)^{1/2} . \tag{104}$$

Note that our dispersion relation (72) is a fourth-order polynomial in $q$, and solving it for a particular choice of $\omega \in \mathbb{C}$ yields four solutions for $q \in \mathbb{C}$. Similarly, a contour in the complex frequency plane $(\omega^{(r)}, \omega^{(i)})$ corresponds to four contours in the complex wavenumber plane $(q^{(r)}, q^{(i)})$, with the latter being referred to as *generalized spatial branches* [20]. For our purposes, we choose frequency contours with constant $\omega^{(i)}$; such contours are denoted $L_\omega$ as in Sec. 3.2.2 of Ref. [20].

For an arbitrary choice of $L_\omega$, the spatial branches will in general not intersect one another. However, when $L_\omega$ passes through $\omega_0$, two spatial branches will pinch, implying the long-time dynamics are influenced by the behavior of both of those branches. To see how the branches pinch, we note that along this particular choice of $L_\omega$, $\omega - \omega_0 = \omega^{(r)} - \omega_0^{(r)}$. By additionally defining $\alpha + \mathrm{i}\beta := (2/\omega''(q_0))^{1/2}$ for notational convenience, with $\alpha$ and $\beta$ being real constants, Eq. $(104)_2$ simplifies to $q - q_0 \approx \pm(\alpha + \mathrm{i}\beta)(\omega^{(r)} - \omega_0^{(r)})^{1/2}$, for which

$$\frac{q^{(i)} - q_0^{(i)}}{q^{(r)} - q_0^{(r)}} = \begin{cases} \pm\dfrac{\beta}{\alpha} & \text{when} \quad \omega^{(r)} - \omega_0^{(r)} > 0 \\[2ex] \mp\dfrac{\alpha}{\beta} & \text{when} \quad \omega^{(r)} - \omega_0^{(r)} < 0 . \end{cases} \tag{105}$$

Accordingly, $q^{(i)} - q_0^{(i)} \propto \pm(q^{(r)} - q_0^{(r)})$ in the vicinity of the saddle point, implying two spatial branches pinch at the saddle point. We therefore seek to characterize the long-time dynamics of the two spatial branches that pinch at the saddle point. To this end, we apply the following procedure, as detailed in Sec. 3.2.2 of Ref. [20]; relevant steps are illustrated in Fig. 4.

1. Choose a value of the Föppl–von Kármán number, with $\Gamma_{\text{test}} > \Gamma_{\text{c}}$, to ensure a temporal instability. In Fig. 4, we chose $\Gamma_{\text{test}} = 0.775 \in \Omega_{\text{A}}$ (left and center columns) and $\Gamma_{\text{test}} = 0.875 \in \Omega_{\text{B}}$ (right column).

2. Calculate the value of $SL_{\text{ac}}(\Gamma_{\text{test}})$ with Eq. (94) if $\Gamma_{\text{test}} \in \Omega_{\text{A}}$ or Eq. (102) if $\Gamma_{\text{test}} \in \Omega_{\text{B}}$. In Fig. 4, the left and center columns correspond to the two values of $SL_{\text{ac}}$ when $\Gamma_{\text{test}} = 0.775 \in \Omega_{\text{A}}$, namely $SL_{\text{ac}}^{-} = 0.056$ and $SL_{\text{ac}}^{+} = 0.063$, while the right column corresponds to $SL_{\text{ac}}^{-}$ when $\Gamma_{\text{test}} = 0.875 \in \Omega_{\text{B}}$.

3. Choose a value of $\omega^{(i)} > \omega_{\text{max}}^{(i)}$, such that $\omega^{(i)}$ is greater than the largest temporal growth rate (75). In Fig. 4, we chose $\omega^{(i)} = 0.05$ in all cases (top row).

4. For the choice of $\omega^{(i)}$, introduce the contour $L_\omega = \omega^{(r)} + \omega^{(i)}$, where $\omega^{(r)}$ varies over $\mathbb{R}$. Solve Eq. (83) for the spatial branches $(q^{(r)}, q^{(i)})$ in the complex wavenumber plane. Due to the choice of $\omega^{(i)}$ in Step 3, no spatial branches can cross the $q^{(r)}$ axis, as doing so would indicate there exists a mode with real $q$ that grows faster than the largest possible growth rate—a contradiction. Thus, the spatial branches lie entirely above or below the $q^{(r)}$ axis. Since $q^{(i)} \neq 0$, the normal modes can be written as

$$\exp\big[\,\mathrm{i}(qz - \omega t)\,\big] = \underbrace{\exp\left[-q^{(i)}\left(z - \frac{\omega^{(i)}}{q^{(i)}}\,t\right)\right]}_{F(z - ct)} \exp\big[\,\mathrm{i}\big(q^{(r)}z - \omega^{(r)}t\big)\,\big] . \tag{106}$$

   As $\omega^{(i)} > 0$, the sign of $q^{(i)}$ determines the sign of $c = \omega^{(i)}/q^{(i)}$ and thus dictates the traveling direction of the spatial branch modes: when $q^{(i)} > 0$, the mode moves to the right, while if $q^{(i)} > 0$ the mode moves to the left. The top row in Fig. 4 shows that in all cases, two modes are right-moving and two modes are left-moving.

5. Continuously select new contours $L_\omega$ as the value of $\omega^{(i)}$ is steadily decreased, until $\omega^{(i)} < 0$; for each $L_\omega$, solve for the four spatial branches $(q^{(r)}, q^{(i)})$ in the complex wavenumber plane. Figure 4 shows how the spatial branches evolve as $\omega^{(i)}$ is lowered from $+0.05$ (top row) to $-0.05$ (bottom row).

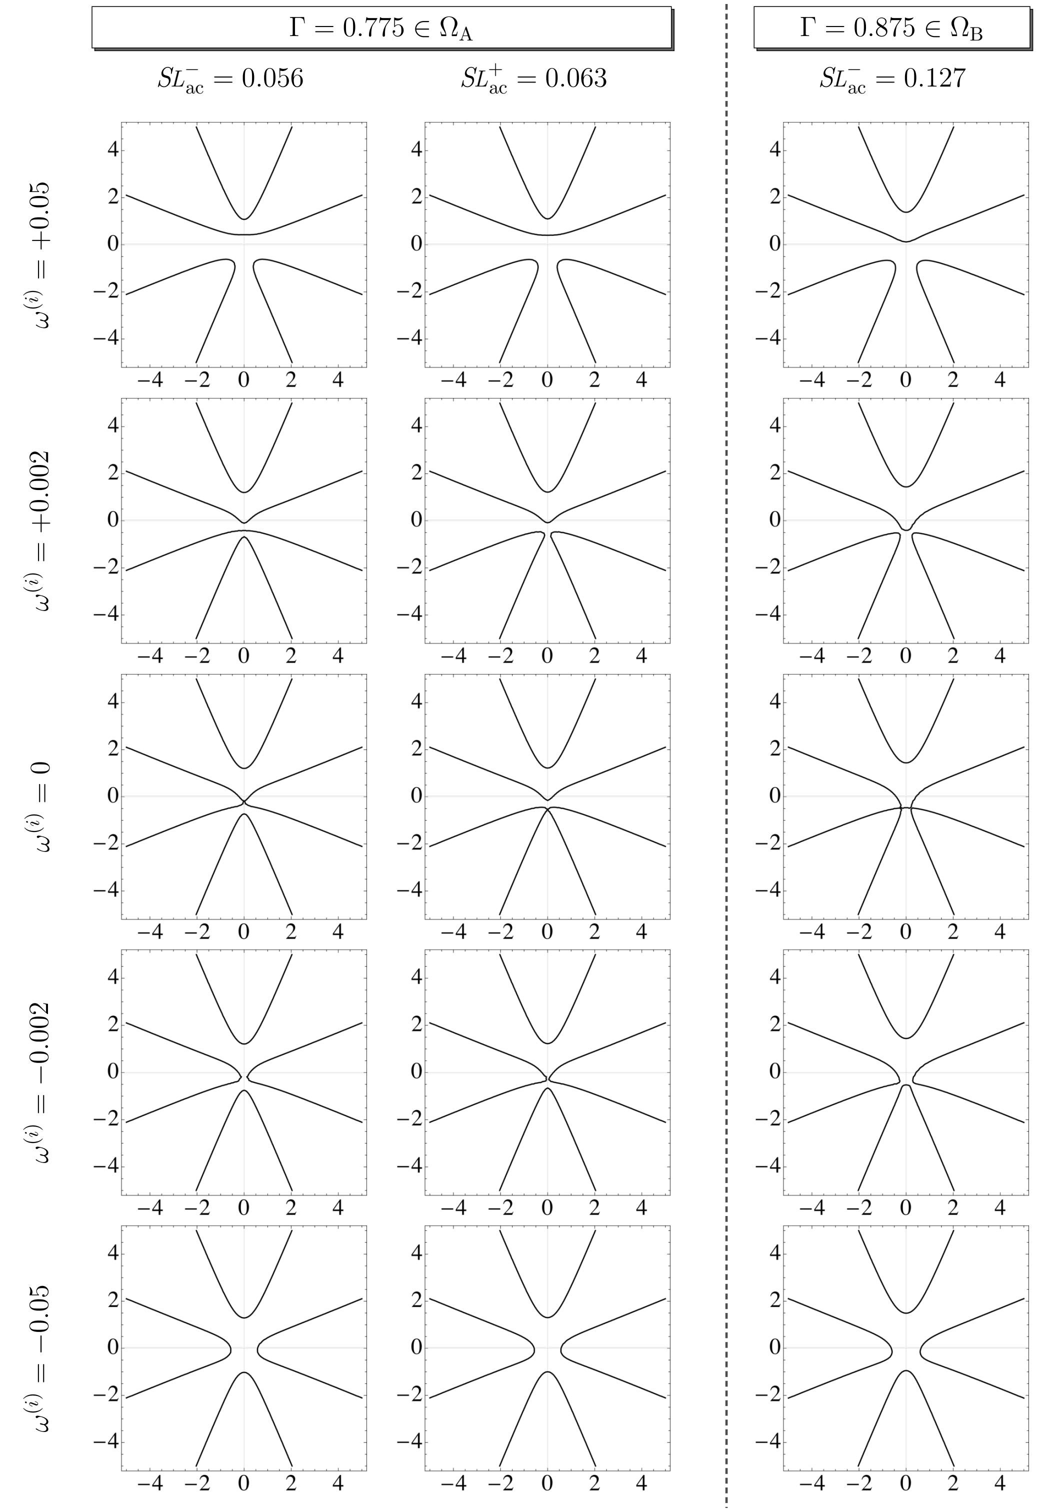


Figure 4: Solution branches in the complex wavenumber plane $(q^{(r)}, q^{(i)})$, for different values of $\omega^{(i)}$. When $\Gamma \in \Omega_A$, two values of $SL_{ac}$ are calculated in Eq. (94), corresponding to the left and center columns. As $\omega^{(i)}$ is decreased, pinching between spatial branches originating from upper and lower half-planes occurs when $SL = SL^-_{ac}$ (left column), but not when $SL = SL^+_{ac}$ (center column). Accordingly, when $\Gamma \in \Omega_A$, only $SL^-_{ac}$ corresponds to a true absolute-to-convective transition. As shown in the right column, when $\Gamma \in \Omega_B$, the value of $SL^-_{ac}$ in Eq. (102) satisfies the pinching criterion.

| | |
|---|---|
| $\Gamma \in \Omega_{\rm A}$ | $g(\Gamma) := -\sqrt{16\Gamma^2 - 104\Gamma + 73}$ <br> $q_0^{(r)} = 0$ <br> $q_0^{(i)} = \dfrac{-1}{2\sqrt{3}}\sqrt{4\Gamma - 1 + g(\Gamma)}$ <br> $\omega_0^{(r)} = 0$ <br> $\omega_0^{(i)} = 0$ <br> $SL_{\rm ac} = \dfrac{8\Gamma - 2 - g(\Gamma)}{48\sqrt{3}}\sqrt{4\Gamma - 1 + g(\Gamma)}$ |
| $\Gamma \in \Omega_{\rm B}$ | $g(\Gamma) := \sqrt{112\Gamma^2 + 136\Gamma - 137}$ <br> $q_0^{(r)\pm} = \pm\dfrac{1}{4}\sqrt{-12\Gamma + 3 + g(\Gamma)}$ <br> $q_0^{(i)} = -\dfrac{1}{4\sqrt{3}}\sqrt{4\Gamma - 1 + g(\Gamma)}$ <br> $\omega_0^{(r)\pm} = \mp\dfrac{12\Gamma - 3 - g(\Gamma)}{48\sqrt{3}}\sqrt{16\Gamma^2 + 40\Gamma - 35 - \frac{1}{2}\big(4\Gamma - 1\big)\,g(\Gamma)}$ <br> $\omega_0^{(i)} = 0$ <br> $SL_{\rm ac} = \dfrac{-8\Gamma + 2 + g(\Gamma)}{48\sqrt{3}}\sqrt{4\Gamma - 1 + g(\Gamma)}$ |

Table 1: Calculated values of the saddle point $(q_0, \omega_0)$ and absolute-to-convective Scriven–Love number $SL_{\rm ac}$, for all $\Gamma > \Gamma_{\rm c}$. When $\Gamma \in \Omega_{\rm A}$, only one of the previously calculated solutions is physically meaningful (see Fig. 4).

6. Monitor how the four spatial branches evolve as $L_\omega$ is lowered in Step 5, paying special attention to the two branches that pinch at $\omega^{(i)} = 0$. As we solved for $SL_{\rm ac}$ with the requirement that $\omega_0^{(i)} = 0$, the branch pinching reveals which spatial branches contribute to the long-time dynamics of the saddle point $(q_0, \omega_0)$. If the pinching branches belonged to different half-planes $q_0^{(i)} > 0$ and $q_0^{(i)} < 0$ for higher $\omega^{(i)}$ (such as in Step 3), then the corresponding modes are moving in different directions and the system is on the verge of losing its sense of directionality—characteristic of an absolute instability. In this case, our calculation of $SL_{\rm ac}(\Gamma_{\rm test})$ indeed corresponds to an absolute-to-convective transition. Otherwise, both modes are traveling in the same direction, and the system is not on the verge of losing its sense of directionality; the saddle point does not represent an absolute-to-convective transition and is thus unphysical.

As we show in Fig. 4, when $\Gamma \in \Omega_{\rm A}$, only the saddle point of absolute wavenumber $q_0 = {\rm i}q_0^{(i)-}$ (93) satisfies the pinching criterion. Therefore, the absolute-to-convective critical speed is given by $SL_{\rm ac}^-$ (94). When $\Gamma \in \Omega_{\rm B}$, the two saddle points of wavenumber $q_0 = q_0^{(r)\pm} + {\rm i}q_0^{(i)}$ (99) simultaneously satisfy the pinching criterion. In this case, the absolute-to-convective critical speed is given by Eq. (102). Our calculation of the physically meaningful saddle point and critical Scriven–Love number, for all $\Gamma > \Gamma_{\rm c}$, is summarized in Table 1.

## 3. Limiting behavior of $\mathit{SL}_{\mathrm{ac}}$

With the calculated values of the Scriven–Love number corresponding to the absolute-to-convective transition, we plot the stability diagram for lipid membrane tubes, in terms of the control parameters $\Gamma$ and $\mathit{SL}$. As shown in Fig. 1(a) in the main text, for every $\Gamma > \Gamma_{\mathrm{c}}$ the tube is absolutely unstable when $\mathit{SL} = 0$. As the Scriven–Love number is increased, the nature of the instability eventually transitions from absolute to convective when $\mathit{SL} = \mathit{SL}_{\mathrm{ac}}(\Gamma)$, such that the system is convectively unstable when $\mathit{SL} > \mathit{SL}_{\mathrm{ac}}$. We now comment on the limiting behavior of the absolute-to-convective Scriven–Love number, $\mathit{SL}_{\mathrm{ac}}$, in two cases: $\Gamma \to \infty$ and $\Gamma \to \Gamma_{\mathrm{c}}^{+}$.

### (a). Limiting behavior when $\Gamma$ is large

An infinite Föppl–von Kármán number corresponds to the limiting case of a two-dimensional fluid film, in which the bending modulus is negligible. For such systems, we take the limit of $\mathit{SL}_{\mathrm{ac}}$ in Table 1, when $\Gamma \in \Omega_{\mathrm{A}}$, and find

$$\lim_{\Gamma\to\infty} \mathit{SL}_{\mathrm{ac}}(\Gamma) = \frac{\Gamma}{2} \,. \tag{107}$$

Interestingly, although Eq. (107) is only valid asymptotically, the result $\mathit{SL}_{\mathrm{ac}} \sim \Gamma/2$ is a reasonable approximation for all $\Gamma > \Gamma_1 \approx 0.801$, as shown in Fig. 1(a) in the main text. However, as $\Gamma$ approaches the instability threshold value of $\Gamma_{\mathrm{c}}$, the approximation breaks down.

### (b). Limiting behavior when $\Gamma$ approaches $\Gamma_{\mathrm{c}}$

As the Föppl–von Kármán number $\Gamma$ approaches $\Gamma_{\mathrm{c}}$, the absolute-to-convective Scriven–Love number can be expanded as the Puiseux series *

$$\mathit{SL}_{\mathrm{ac}} = \frac{\sqrt{2}}{4}\left(\Gamma - \Gamma_{\mathrm{c}}\right)^{1/2} - \frac{\sqrt{2}}{2}\left(\Gamma - \Gamma_{\mathrm{c}}\right)^{5/2} - 4\sqrt{2}\left(\Gamma - \Gamma_{\mathrm{c}}\right)^{7/2} + \dots \,. \tag{108}$$

Thus, close to the instability threshold, one may approximate $\mathit{SL}_{\mathrm{ac}}$ as

$$\mathit{SL}_{\mathrm{ac}} \approx \frac{\sqrt{2}}{4}\left(\Gamma - \Gamma_{\mathrm{c}}\right)^{1/2} \qquad \text{for} \qquad \Gamma \to \Gamma_{\mathrm{c}}^{+} \,. \tag{109}$$

As shown in the inset in Fig. 1(a) of the main text, Eq. (109) is a reasonable approximation for $\Gamma$ between $\Gamma_{\mathrm{c}}$ and $\Gamma_1$. Over this range, $\Gamma \in \Omega_{\mathrm{A}}$, such that $q_0$ is purely imaginary and $\omega_0$ is identically zero at the absolute-to-convective transition (see Table 1). The square root dependence seen in Eq. (109), as well as the relations $q_0^{(r)} = 0$ and $\omega_0^{(r)} = 0$, are reminiscent of the well-studied GL equation. For a general scalar field $\phi \in \mathbb{R}$ and constant real control parameters $u$ and $\kappa$, the linearized GL equation is given by

$$\phi_{,t} + u\,\phi_{,x} = \kappa\,\phi + \phi_{,xx} \,. \tag{110}$$

It is well-known that Eq. (110) is unstable when $\kappa > 0$, and undergoes an absolute-to-convective transition for $u_{\mathrm{ac}} = 2\kappa^{1/2}$ [20]. At this point, we recall the linearized evolution equation for the perturbed membrane radius $\tilde{r}$ (58)—which is similar in structure to the linearized GL equation (110). The important difference is the $\tilde{r}_{,zzzz}$ term arising from the $-k_{\mathrm{b}}\Delta_{\mathrm{s}}H$ term in the shape equation (4). As such, Eq. (58) belongs to the family of so-called extended Fisher–Kolmogorov (EFK) equations [27–29]. Nonetheless, our present task is to show the last term in Eq. (58) is negligible in the limit $\Gamma \to \Gamma_{\mathrm{c}}$—thus showing how the rich set of behaviors predicted by the GL equation is relevant in understanding the dynamics of lipid membrane tubes.

We start by noting the fourth-order term is not the only bending term in Eq. (58): both $-(\Gamma_{\mathrm{c}}/4)\,\tilde{r}$ and $-(\Gamma_0/4)\,\tilde{r}_{,zz}$ originate from bending forces as well. While $\tilde{r}_{,zzzz}$ is negligible when $\Gamma \to \infty$, in this limit the other bending terms are also unimportant, thus yielding $\mathit{SL}_{\mathrm{ac}} \sim \Gamma/2$, as discussed previously. In the limit where $\Gamma \to \Gamma_{\mathrm{c}}$, however, the crucial insight is that the marginally stable wavenumber goes to zero as $q_{\mathrm{ms}} \sim (\Gamma - \Gamma_{\mathrm{c}})^{1/2}$ [see Eq. (76)], such that only long wavelength perturbations are unstable. Since the

*This series expansion was obtained using `Mathematica`.

dominant wavenumbers are those for which $q < q_{\text{ms}}$, the various contributions on the right hand side of Eq. (58) scale at most as

$$\left(\frac{\Gamma - \Gamma_{\text{c}}}{4}\right)\tilde{r} \sim (\Gamma - \Gamma_{\text{c}}) \ , \qquad \left(\frac{\Gamma - \Gamma_0}{4}\right)\tilde{r}_{,zz} \sim (\Gamma_{\text{c}} - \Gamma_0)(\Gamma - \Gamma_{\text{c}}) \ , \qquad \text{and} \qquad -\frac{1}{8}\,\tilde{r}_{,zzzz} \sim (\Gamma - \Gamma_{\text{c}})^2 \tag{111}$$

as $\Gamma$ approaches $\Gamma_{\text{c}}$. In this limit, the $\tilde{r}_{,zzzz}$ term is negligible relative to the other terms, and Eq. (58) simplifies to

$$\tilde{r}_{,t} + \mathit{SL}\,\tilde{r}_{,z} = \left(\frac{\Gamma - \Gamma_{\text{c}}}{4}\right)\tilde{r} + \left(\frac{\Gamma - \Gamma_0}{4}\right)\tilde{r}_{,zz} \qquad \text{as} \qquad \Gamma \to \Gamma_{\text{c}}^{+} \ . \tag{112}$$

Equation (112) can be recast in a similar form to the linearized GL equation (110) with the change of variables $x = 2z(\Gamma - \Gamma_0)^{-1/2}$, for which Eq. (112) becomes

$$\tilde{r}_{,t} + \left(\frac{2\,\mathit{SL}}{\sqrt{\Gamma - \Gamma_0}}\right)\tilde{r}_{,x} = \left(\frac{\Gamma - \Gamma_{\text{c}}}{4}\right)\tilde{r} + \tilde{r}_{,xx} \qquad \text{as} \qquad \Gamma \to \Gamma_{\text{c}}^{+} \ . \tag{113}$$

In the limit of $\Gamma \to \Gamma_{\text{c}}$, our parameters can be related to those in the linearized GL equation (110) by $u = 2\mathit{SL}(\Gamma - \Gamma_0)^{-1/2}$ and $\kappa = (\Gamma - \Gamma_{\text{c}})/4$. As the GL equation is unstable when $\kappa > 0$ and undergoes an absolute-to-convective transition when $u_{\text{ac}} = 2\kappa^{1/2}$, we expect our membrane system to be unstable when $\Gamma > \Gamma_{\text{c}}$ and undergo an absolute-to-convective transition when $\mathit{SL}_{\text{ac}} = \frac{1}{2}(\Gamma - \Gamma_0)^{1/2}(\Gamma - \Gamma_{\text{c}})^{1/2} \approx \frac{\sqrt{2}}{4}(\Gamma - \Gamma_{\text{c}})^{1/2}$ as $\Gamma \to \Gamma_{\text{c}}$, which agrees with the prediction of the series expansion in Eq. (108).

## 4. Numerical solutions of linearized dynamics

We conclude our linear analysis of unstable lipid membrane tubes by presenting results from numerical simulations, which confirm our theoretical predictions of the absolute-to-convective transition. We first describe our numerical method to solve for the evolving membrane shape over time, as predicted by the linear theory, and then show the space–time evolution of an unstable, axisymmetric tube which is locally perturbed.

An axisymmetric lipid membrane tube is described by three fundamental unknowns, namely the perturbed shape $\tilde{r}(z,t)$, surface tension $\tilde{\lambda}(z,t)$, and in-plane axial velocity $\tilde{v}^z(z,t)$. The three corresponding governing equations can be combined into a single evolution equation for $\tilde{r}$, as presented in Eq. (58). Thus, to solve for the membrane shape over time according to the linearized dynamics, we need only to solve Eq. (58) numerically. To this end, we observe that as $\Gamma$ increases, $\mathit{SL}_{\text{ac}}(\Gamma)$ increases as well. Accordingly, when the Föppl–von Kármán number is large, we seek to simulate systems with a large base flow to observe the absolute-to-convective transition. In this case, to ensure the disturbance does not flow past the edge of our computational domain, a large spatial domain is required. To avoid this numerical inconvenience, we introduce the rescaled variables

$$T = \left(\frac{\Gamma - \Gamma_{\text{c}}}{4}\right)t \qquad \text{and} \qquad Z = \left(\frac{\Gamma - \Gamma_{\text{c}}}{\Gamma - \Gamma_0}\right)^{1/2} z \ , \tag{114}$$

which are only physically meaningful when $\Gamma > \Gamma_{\text{c}}$; note that rescaling time by $(\Gamma - \Gamma_{\text{c}})$ and space by $(\Gamma - \Gamma_{\text{c}})^{1/2}$ is a common technique when studying universality properties of the GL equation [30]. By substituting Eq. (114) into the linearized evolution equation (58), and recognizing the Scriven–Love number is correspondingly rescaled as

$$\overline{\mathit{SL}} = \frac{4\,\mathit{SL}}{(\Gamma - \Gamma_{\text{c}})^{1/2}\,(\Gamma - \Gamma_0)^{1/2}} \ , \tag{115}$$

we obtain

$$\tilde{r}_{,T} + \overline{\mathit{SL}}\,\tilde{r}_{,Z} = \tilde{r} + \tilde{r}_{,ZZ} - \frac{1}{2}\frac{(\Gamma - \Gamma_{\text{c}})}{(\Gamma - \Gamma_0)^2}\,\tilde{r}_{,ZZZZ} \ . \tag{116}$$

Importantly, in the absence of spatial variations, Eq. (116) simplifies to $\tilde{r}_{,T} = \tilde{r}$, such that the growth rate is independent of the Föppl–von Kármán number. Moreover, the rescaled absolute-to-convective Scriven–Love number $\overline{\mathit{SL}}_{\text{ac}}$ is of order unity for all unstable $\Gamma$. Consequently, we may now use the same spatial and temporal domains for all simulations.

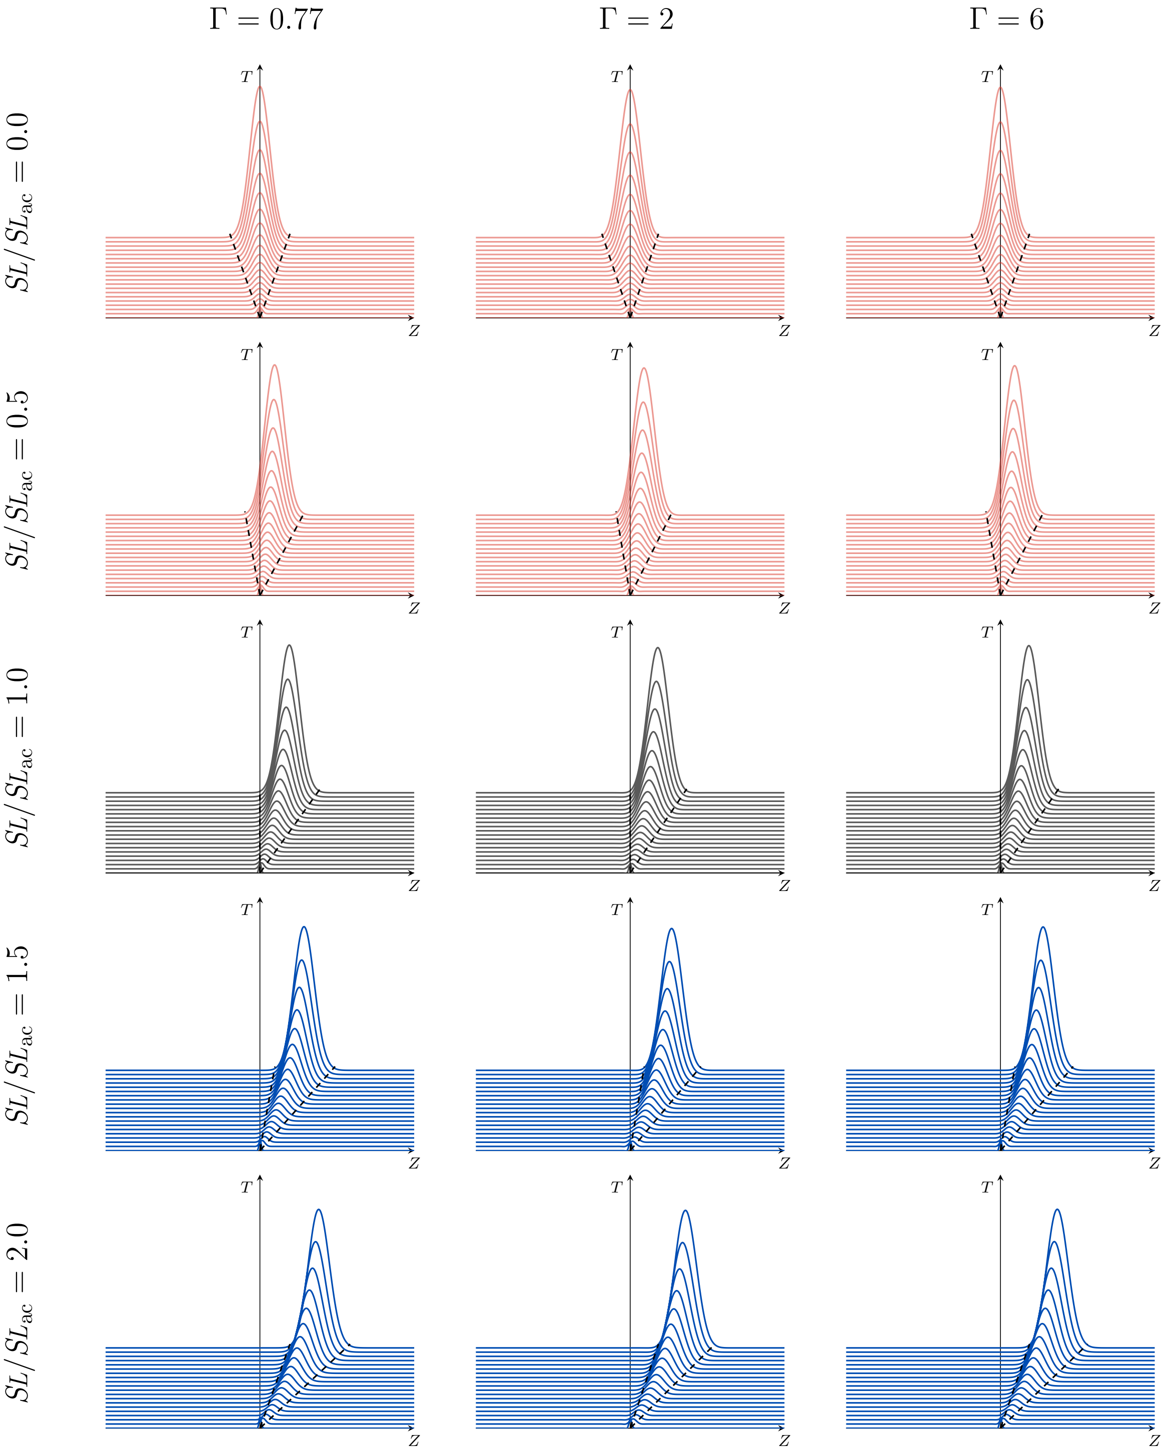


Figure 5: Space–time plots showing snapshots of the tube profile at different instants and for different values of the control parameters. From left to right, $\Gamma = 0.77$, 2, and 6; from top to bottom, $SL/SL_{\mathrm{ac}} = 0$, 0.5, 1, 1.5, and 2. The dashed black lines show the edges of the growing wavepacket and were obtained by determining the propagation speed of a front invading an unstable tube [see Eq. (123)].

The results of our numerical simulations, in terms of the rescaled variables $Z$ and $T$, are shown in Fig. 5. All simulations were run on the fixed domain $Z \in [-50, 50]$ and with the initial condition $\tilde{r}(Z, 0) = 0.1 \exp\left(-10Z^2\right)$. We chose three different Föppl–von Kármán numbers: $\Gamma = 0.77 \in (\Gamma_c, \Gamma_1)$, $\Gamma = 2 \in (\Gamma_1, \Gamma_2)$, and $\Gamma = 6 > \Gamma_2$. For each choice of $\Gamma$, simulations were carried out at five values of the Scriven–Love number: $\overline{SL}/\overline{SL}_{\rm ac} = SL/SL_{\rm ac} = 0$, 0.5, 1, 1.5, and 2, which were chosen such that we sampled (i) absolutely unstable systems, (ii) convectively unstable systems, and (iii) systems at the transition between the two. As shown in Fig. 5, our numerical results confirm our theoretical calculation of $SL_{\rm ac}$. When $SL < SL_{\rm ac}$, the instability grows to invade the entire domain, while if $SL > SL_{\rm ac}$ then a stationary observer downstream will see a transient growth followed by a decay at long times. Moreover, our simulations show that as an initial perturbation grows, its edges propagate outward and invade the unstable tube at a constant velocity (see the dashed lines in Fig. 5). In all cases, the velocity of the leading edge is positive; however the velocity of the trailing edge is negative when $SL < SL_{\rm ac}$, zero when $SL = SL_{\rm ac}$, and positive when $SL > SL_{\rm ac}$. In the following section, we investigate the dynamics of the moving fronts via linear methods.

## 5. Speed of propagating fronts: Marginal stability criterion

To determine the speed at which an initially local perturbation invades the neighboring unperturbed tube, we apply the classical marginal stability criterion (MSC) [31–33]—one of the many well-established techniques for studying front propagation. Consider an initially localized wavepacket consisting of perturbations of the form $\sim\exp[\mathrm{i}(qz - \omega t)]$, which is growing and spreading in an unstable system. If an observer is moving at a speed slightly greater than the front velocity $V_{\rm f}$, they will see an unperturbed tube as they remain ahead of the growing wavepacket. If, on the other hand, an observer moves slightly slower than the front velocity, they will then see the tube changing shape: either growing or decaying, based on the sign of the growth rate in the traveling frame. The MSC hypothesis states that the front speed is that for which an observer traveling at speed $V_{\rm f}$ would see the system in its marginal state, i.e. on the verge of being deformed. Thus, in the reference frame of the front connecting the deformed and undeformed regions of the tube, an observer perceives perturbations of zero growth rate.

In terms of our dimensionless quantities, the front velocity $V_{\rm f}$ is captured by what we call the Scriven–Love number of the front, $SL_{\rm f} := \zeta V_{\rm f} r_0 / k_{\rm b}$. In the reference frame of the front, the Doppler-shifted axial position and frequency are respectively given by

$$z^\dagger = z - SL_{\rm f}\, t \qquad \text{and} \qquad \omega^\dagger = \omega - SL_{\rm f}\, q \ , \tag{117}$$

such that a mode in our wave packet can be expressed as [c.f. Eq. (59)]

$$\exp\left\{\mathrm{i}\left[qz - \omega t\right]\right\} = \exp\left\{\mathrm{i}\left[q\left(z^\dagger + SL_{\rm f}\, t\right) - \left(\omega^\dagger + SL_{\rm f}\, q\right)t\right]\right\} = \exp\left\{\mathrm{i}\left[qz^\dagger - \omega^\dagger t\right]\right\} \ . \tag{118}$$

The MSC is then given by

$$\omega^{\dagger(i)} = 0 \ . \tag{119}$$

We additionally note that in the reference frame of the front, i.e. the frame in which the front is stationary, the edge of the wavepacket invading the unperturbed tube is traveling at zero group velocity—for which

$$\left.\frac{\mathrm{d}\omega^\dagger}{\mathrm{d}q}\right|_{q_{\rm f}} = 0 \ , \qquad \text{thus requiring} \qquad \mathrm{Re}\left\{\left.\frac{\mathrm{d}\omega^\dagger}{\mathrm{d}q}\right|_{q_{\rm f}}\right\} = 0 \qquad \text{and} \qquad \mathrm{Im}\left\{\left.\frac{\mathrm{d}\omega^\dagger}{\mathrm{d}q}\right|_{q_{\rm f}}\right\} = 0 \ . \tag{120}$$

In Eq. (120), $q_{\rm f}$ is the wavenumber associated with the front, which characterizes spatial oscillations at the point where the wavepacket invades the unperturbed tube.

With Eq. (119), the two conditions in Eq. (120), and the real and imaginary components of the dispersion relation $\omega^\dagger_{\rm f} = \omega(q_{\rm f}) - SL_{\rm f}\, q_{\rm f}$ $(117)_2$, we have five equations which solve for the five unknowns $q_{\rm f}^{(r)}$, $q_{\rm f}^{(i)}$, $\omega_{\rm f}^{\dagger(r)}$, $\omega_{\rm f}^{\dagger(i)}$, and $SL_{\rm f}$ in terms of the Föppl–von Kármán number $\Gamma$. Note that when calculating $\omega(q_{\rm f})$ via the dispersion relation (72), the Scriven–Love number $SL$ is in general not equal to the dimensionless front velocity $SL_{\rm f}$. Interestingly, the system of equations under consideration is almost identical to those in the absolute/convective analysis, in which the saddle point $(q_0, \omega_0)$ is replaced by $(q_{\rm f}, \omega_{\rm f})$—the one exception being that before, $\omega_0 = SL\, q_0 + \mathrm{i}[\ldots]$ (72) while now, $\omega_{\rm f}^\dagger = (SL - SL_{\rm f})q_{\rm f} + \mathrm{i}[\ldots]$ (117). In this case, the front wavenumber $q_{\rm f}$ is nearly identical to the absolute wavenumber $q_0$, with one important difference. In

particular, as discussed below Eq. (92), we limited physically meaningful absolute wavenumbers to those with negative imaginary components, such that our spatial ansatz grew downstream, in the direction of the base flow. In this case, however, fronts can propagate in either direction (regardless of the base flow direction), so we place no restrictions on the sign of $q_{\mathrm{f}}^{(i)}$. Accordingly, the real and imaginary components of the front wavenumber are given by (cf. Table 1)

$$q_{\mathrm{f}}^{(r)} = 0 \qquad \text{and} \qquad q_{\mathrm{f}}^{(i)} = \frac{\pm 1}{2\sqrt{3}} \sqrt{4\Gamma - 1 + g(\Gamma)} \qquad \text{when} \qquad \Gamma \in \Omega_{\mathrm{A}} \ , \tag{121}$$

and

$$q_{\mathrm{f}}^{(r)} = \pm \frac{1}{4} \sqrt{-12\Gamma + 3 + g(\Gamma)} \qquad \text{and} \qquad q_{\mathrm{f}}^{(i)} = \frac{\pm 1}{4\sqrt{3}} \sqrt{4\Gamma - 1 + g(\Gamma)} \qquad \text{when} \qquad \Gamma \in \Omega_{\mathrm{B}} \ , \tag{122}$$

where $g(\Gamma)$ is defined in Table 1. As can be seen from Eq. (80) in the saddle point analysis, the '$\pm$' prefactor of $q_{\mathrm{f}}^{(i)}$ in Eqs. (121) and (122) leads to the analogous result $SL - SL_{\mathrm{f}} = \pm SL_{\mathrm{ac}}$, such that the leading and trailing dimensionless front velocities, $SL_{\mathrm{f}}^{+}$ and $SL_{\mathrm{f}}^{-}$, are respectively given by

$$SL_{\mathrm{f}}^{+} = SL + SL_{\mathrm{ac}} \qquad \text{and} \qquad SL_{\mathrm{f}}^{-} = SL - SL_{\mathrm{ac}} \ , \tag{123}$$

where $SL_{\mathrm{ac}}$ is provided in Table 1 for all values of $\Gamma > \Gamma_{\mathrm{c}}$. Equation (123) is consistent with our observations from Fig. 5: the velocity of the trailing front determines if the system is (i) absolutely unstable, with $SL_{\mathrm{f}}^{-} < 0$, (ii) convectively unstable, with $SL_{\mathrm{f}}^{-} > 0$, or (iii) at the absolute-to-convective transition, with $SL_{\mathrm{f}}^{-} = 0$.

As briefly mentioned in the main text, Eq. (123) can qualitatively explain previous findings from an experimental study, in which the speed of front propagation in lipid membrane tubes was measured at different values of the base tension [34]. In these experiments, the membrane tubes were initially at rest, such that $SL = 0$. The front speed was observed to vary linearly with the rescaled tension, $(\Gamma - \Gamma_{\mathrm{c}})/\Gamma_{\mathrm{c}}$, everywhere except at tensions very close to the critical tension. Moreover, over this linear regime, the MSC was successfully used to explain the front propagation speed. However, when $\Gamma$ approached $\Gamma_{\mathrm{c}}$, the previous study fitted their data to a decaying exponential without further explanation. However, we now understand the decay of the front speed close to the instability threshold via Eq. (123). As both leading and trailing fronts travel with speed $SL_{\mathrm{ac}}$ when there is no base flow, we expect the front velocity to scale as $SL_{\mathrm{f}} \sim (\Gamma - \Gamma_{\mathrm{c}})^{1/2}$ close to the threshold. We hope such a prediction motivates further careful experiments close to the instability threshold, in which $\Gamma \in [\Gamma_{\mathrm{c}}, \Gamma_1]$.

The above comparison with experimental data highlights the importance of the Föppl–von Kármán number $\Gamma_1$ in separating different regimes of the front velocity. However, we have not yet commented on the physical significance of $\Gamma_1$, its counterpart $\Gamma_2$, or the intervals $\Omega_{\mathrm{A}}$ and $\Omega_{\mathrm{B}}$. In what follows, we conclude our linear spatiotemporal analysis by discussing the physics of these particular values of the Föppl–von Kármán number, and the resultant domains between them.

## 6. Understanding $\Gamma_1$ and $\Gamma_2$ as Lifshitz points

Results from our application of the MSC to unstable membrane tubes are captured by Eqs. (121) and (122), which are informative as to the nature of $\Gamma_1$ and $\Gamma_2$. In particular, both the front wavenumber $q_{\mathrm{f}}$ and frequency $\omega_{\mathrm{f}}$ bifurcate at $\Gamma = \Gamma_1$ (see Fig. 2 in the main text): as $\Gamma$ is increased through $\Gamma_1$, the deformations accompanying the moving fronts transition from being monotonic ($q_{\mathrm{f}}^{(r)} = 0$) to being spatially oscillatory ($q_{\mathrm{f}}^{(r)} \neq 0$). The opposite scenario occurs at $\Gamma_2$, as $q_{\mathrm{f}}$ and $\omega_{\mathrm{f}}$ again bifurcate, but in this case the front transitions from oscillatory to monotonic as $\Gamma$ is increased. Such bifurcations in the wavenumber of the emerging state are reminiscent of the so-called Lifshitz points (LPs) first introduced in the context of phase transitions [35,36], at which the lowest-order gradient term in the free energy vanishes. The analogy between LPs and steady-to-oscillatory bifurcations was previously made in investigations of the EFK equation, for which the $q^2$ term in the dispersion relation vanishes at the saddle point [37,38]. In the case of lipid membrane tubes, we show $\Gamma_1$ and $\Gamma_2$ are LPs by first recalling that at long times, the dispersion relation in the reference frame of the front can be approximated by

$$\omega^{\dagger} \approx \omega_{\mathrm{f}}^{\dagger} + \frac{1}{2} \frac{\mathrm{d}^2 \omega^{\dagger}}{\mathrm{d}q_{\mathrm{f}}^2}\bigg|_{q_{\mathrm{f}}} (q - q_{\mathrm{f}})^2 \ , \tag{124}$$

where $\omega_{\mathrm{f}}^{\dagger} := \omega^{\dagger}(q_{\mathrm{f}})$ and $(\mathrm{d}\omega^{\dagger}/\mathrm{d}q)|_{q_{\mathrm{f}}} = 0$ from Eq. (120). In what follows, we show that when $\Gamma = \Gamma_1$ and $\Gamma = \Gamma_2$, the right hand side of this approximation vanishes—demonstrating that $\Gamma_1$ and $\Gamma_2$ are Lifshitz points. To this end, recall that by definition, $\omega_{\mathrm{f}}^{\dagger} = \omega_{\mathrm{f}}^{\dagger(r)}$ according to the MSC (119), and thus

$$\omega_{\mathrm{f}}^{\dagger}(\Gamma) \; = \; 0 \qquad \text{at} \quad \Gamma = \Gamma_1 \;\; \text{and} \;\; \Gamma = \Gamma_2 \; . \tag{125}$$

Next, we recognize that Eq. $(117)_2$ implies $\mathrm{d}^2\omega^{\dagger}/\mathrm{d}q^2 = \mathrm{d}^2\omega/\mathrm{d}q^2$; by differentiating the dispersion relation Eq. (72) twice, we obtain

$$\frac{\mathrm{d}^2\omega^{\dagger}}{\mathrm{d}q^2}\bigg|_{q_{\mathrm{f}}} \; = \; -\frac{\mathrm{i}}{8}\Big(4\Gamma - 1 + 12q_{\mathrm{f}}^2\Big) \; . \tag{126}$$

To calculate the front wavenumber $q_{\mathrm{f}}$, we note that $\Omega_{\mathrm{A}}$ and $\Omega_{\mathrm{B}}$ coincide at $\Gamma = \Gamma_1$ and $\Gamma = \Gamma_2$, and the front wavenumber coincides at these values of the Föppl–von Kármán number as well. We find that in $\Omega_{\mathrm{A}}$, where $g(\Gamma) = -\sqrt{16\Gamma^2 - 104\Gamma + 73}$, $g(\Gamma_1) = g(\Gamma_2) = 0$; consequently, Eq. (121) simplifies to $q_{\mathrm{f}} = \mathrm{i}\sqrt{(4\Gamma - 1)/12}$ at $\Gamma_1$ and $\Gamma_2$. Substituting this result into Eq. (126) yields

$$\frac{\mathrm{d}^2\omega^{\dagger}}{\mathrm{d}q^2}\bigg|_{q_{\mathrm{f}}} \; = \; -\frac{\mathrm{i}}{8}\Big(4\Gamma - 1 - 12\big(q_{\mathrm{f}}^{(i)}\big)^2\Big) \; = \; 0 \qquad \text{at} \quad \Gamma = \Gamma_1 \;\; \text{and} \;\; \Gamma = \Gamma_2 \; . \tag{127}$$

With Eqs. (124), (125), and (127), we find that at $\Gamma = \Gamma_1$ and $\Gamma = \Gamma_2$, the usual long-time approximation of the dispersion relation is insufficient. Accordingly, $\Gamma_1$ and $\Gamma_2$ are identified as LPs, for which the expansion in Eq. (124) needs to be supplemented with higher order terms for a correct first approximation of the front dynamics. We thus find

$$\omega^{\dagger} \; \approx \; \frac{1}{6}\,\frac{\mathrm{d}^3\omega^{\dagger}}{\mathrm{d}q_{\mathrm{f}}^3}\bigg|_{q_{\mathrm{f}}} \big(q - q_{\mathrm{f}}\big)^3 \; = \; -\frac{\mathrm{i}}{2}\, q_{\mathrm{f}}\,\big(q - q_{\mathrm{f}}\big)^3 \qquad \text{at} \quad \Gamma = \Gamma_1 \;\; \text{and} \;\; \Gamma = \Gamma_2 \; . \tag{128}$$

Our finding that $\Gamma_1$ and $\Gamma_2$ are LPs is consistent with prior investigations of front propagation in the EFK equation. In particular, Refs. [37, 38] found a single LP describing a steady-to-oscillatory bifurcation when the coefficient of the fourth-order term, denoted $\gamma$, crossed a critical value of $\gamma = \gamma_{\mathrm{c}} = {}^1\!/_{12}$. Interestingly, as discussed in the main text, when mapping the linearized membrane evolution equation (58) to the usual form of the EFK equation (e.g. that in Ref. [31]), we find $\gamma = (\Gamma - \Gamma_{\mathrm{c}})/(\Gamma - \Gamma_0)^2$, such that both $\Gamma_1$ and $\Gamma_2$ correspond to the previously obtained critical value of $\gamma_{\mathrm{c}} = {}^1\!/_{12}$.

# IV. Nonlinear dynamics

In the above simulations of linearized membrane dynamics, we found initially localized perturbations grow and invade the undeformed tube via propagating fronts. Moreover, in this case we found the front speed was characterized by the MSC theory [19, 39]. Our results corroborate the observation that front propagation causes shape deformations in both biological and in vitro systems, such as neurons [13] and membrane tethers [10, 34]. However, the linearized simulations do not contain nonlinear saturating effects—which, in experimental systems, would eventually dominate the unstable behavior. In this section, we investigate the nonlinear dynamics of lipid membrane tubes by performing fully nonlinear simulations under axisymmetric conditions. Furthermore, in order to understand the mechanisms at play during the nonlinear stages of the instability, we develop a weakly nonlinear model for membrane tubes that extends Eq. (116) into a nonlinear EFK equation by retaining some nonlinearities from the axisymmetric equations (31)–(33). The approximate EFK equation is useful in that it (i) provides a simplified physical understanding of nonlinearities in the system, and (ii) is straightforward to solve numerically. The robustness of this weakly nonlinear model is then tested by comparing its predictions to results from fully nonlinear simulations.

## 1. Weakly nonlinear analysis

First, we derive a weakly nonlinear model for the dynamics of lipid membrane tubes by retaining some, but not all, nonlinearities of the general governing equations. In particular, we keep nonlinear terms which are

algebraic in the perturbed radius, but neglect terms involving products of derivatives, as will be described in detail below. Under this assumption, we first simplify the general axisymmetric equations presented in Sec. I.3 (b) and then condense the governing equations into a single weakly nonlinear evolution equation for the membrane shape.

To begin, for an axisymmetric lipid membrane in one-to-one correspondence with an unperturbed cylinder and parametrized as in Eq. (26), membrane dynamics are governed by Eqs. (31)–(33). While the general equations are too complex to be treated analytically, we now seek a description which both maintains some of the nonlinearities and is also analytically tractable. To this end, we simplify the problem by assuming the perturbed shape is weakly varying, such that derivatives of $r$ are small. Defining $\partial_z^j\, r := \partial^j r/\partial z^j$, we express our assumption mathematically as

$$\partial_z^j\, r \,*\, \partial_z^k\, r \quad \text{is} \quad \begin{cases} \text{negligible if } j \geq 1 \text{ and } k \geq 1 \\ \text{non-negligible otherwise} \;. \end{cases} \tag{129}$$

We additionally assume that spatial gradients in the membrane are weakly coupled to its temporal evolution, for which

$$r_{,t} \,*\, \partial_z^j\, r \quad \text{is} \quad \begin{cases} \text{negligible if } j \geq 1 \\ \text{non-negligible otherwise} \;. \end{cases} \;. \tag{130}$$

With Eq. (129), our previously calculated value of $a_{22} = 1 + r_{,z}^2$ in Eq. (28) simplifies to one; the mean curvature, Gaussian curvature, and nonzero Christoffel symbols are then given by [cf. Eqs. (29) and (30)]

$$\begin{aligned} H \;&=\; -\frac{1}{2r}\left(1 - r\, r_{,zz}\right) \;, & K \;&=\; -\frac{r_{,zz}}{r} \;, \\ \Gamma^1_{12} \;=\; \Gamma^1_{21} \;&=\; \frac{r_{,z}}{r} \;, \qquad \text{and} & \Gamma^2_{11} \;&=\; -r r_{,z} \;. \end{aligned} \tag{131}$$

By substituting Eq. (131) into Eqs. (31)–(33) and applying the weakly nonlinear assumptions in Eqs. (129) and (130), we obtain the governing equations

$$r v^z_{,z} \,+\, r_{,z} v^z \,+\, r_{,t} \;=\; 0 \;, \tag{132}$$

$$-\, 2\zeta \left( r_{,zt} \,+\, v^z\, r_{,zz} \right) \,+\, r \lambda_{,z} \;=\; 0 \;, \tag{133}$$

and

$$p \,+\, \lambda \left( r_{,zz} \,-\, \frac{1}{r} \right) \,+\, 2\zeta \left( v^z_{,z}\, r_{,zz} \,-\, \frac{v^z\, r_{,z}}{r^2} \,-\, \frac{r_{,t}}{r^2} \right) \,-\, k_{\mathrm{b}} \left( \frac{-1}{4r^3} \,+\, \frac{r_{,zz}}{4r^2} \,+\, \frac{1}{2}\, r_{,zzzz} \right) \;=\; 0 \;, \tag{134}$$

where the continuity equation (132) was used to simplify the form of the shape equation (134).

While Eqs. (132)–(134) constitute three equations for the three unknowns $v^z$, $\lambda$, and $r$, we have not yet commented on the magnitude of the in-plane velocity or surface tension. To this end, we expand both quantities as

$$v^z(z,t) \;=\; v^z_{(0)} \,+\, v^z_{(1)}(z,t) \qquad \text{and} \qquad \lambda(z,t) \;=\; \lambda_{(0)} \,+\, \lambda_{(1)}(z,t) \;, \tag{135}$$

where $v^z_{(0)}$ and $\lambda_{(0)}$ are assumed to be constant quantities. In Eq. (135), we do not introduce the small parameter $\epsilon$, and therefore employ a different notation from that in the linearized theory (41). We now make the two additional assumptions that

$$v^z_{(1)} \,*\, \partial_z^j\, r \qquad \text{and} \qquad \lambda_{(1)} \,*\, \partial_z^j\, r \quad \text{are} \quad \begin{cases} \text{negligible if } j \geq 1 \\ \text{non-negligible otherwise} \;, \end{cases} \tag{136}$$

in a manner consistent with our previous assumptions (129 and 130). With Eqs. (135) and (136), the in-plane equation (133) becomes

$$-\, 2\zeta \left( r_{,zt} \,+\, v^z_{(0)}\, r_{,zz} \right) \,+\, r\, \lambda_{(1),z} \;=\; 0 \;. \tag{137}$$

We simplify the second term in Eq. (137) by recognizing

$$r\, \lambda_{(1),z} \;=\; \left( r\, \lambda_{(1)} \right)_{,z} \,-\, r_{,z}\, \lambda_{(1)} \;\approx\; \left( r\, \lambda_{(1)} \right)_{,z} \;, \tag{138}$$

where Eq. (136) was used in the last step. Equation (137) can then be integrated in $z$ to yield

$$-\,2\zeta\left(r_{,t}\,+\,v^{z}_{(0)}\,r_{,z}\right)\,+\,r\,\lambda_{(1)}\;=\;c(t)\;, \tag{139}$$

for some integration constant $c(t)$. However, we assume perturbed quantities go to zero as $z \to \infty$, such that $c(t) = 0$, in which case the perturbed surface tension is given by

$$\lambda_{(1)}\;=\;\frac{2\zeta}{r}\left(r_{,t}\,+\,v^{z}_{(0)}\,r_{,z}\right)\;. \tag{140}$$

According to Eq. (140), the perturbed surface tension can be calculated from the evolution of the membrane shape over time.

To obtain the perturbed shape equation, we first recognize the base state membrane equations require $p = \lambda_{(0)}/r_0 - k_b/(4r_0^3)$ [see Eq. (53)]. By substituting this expression for the pressure, as well as Eq. (140), into Eq. (134), simplifying with our assumptions in Eqs. (129) and (136), and rearranging terms, we obtain

$$\frac{4r_0^2}{r^2}\left(\frac{\zeta\,r_0}{k_b}\,r_{,t}\,+\,\frac{\zeta\,v^{z}_{(0)}\,r_0}{k_b}\,r_{,z}\right)\;=\;\frac{r_0^2\,\lambda_{(0)}}{k_b}\left(1\,-\,\frac{r_0}{r}\,+\,r_0\,r_{,zz}\right)\,-\,\frac{1}{4}\left(1\,-\,\frac{r_0^3}{r^3}\,+\,\frac{r_0^3\,r_{,zz}}{r^2}\,+\,2r_0^3\,r_{,zzzz}\right)\,. \tag{141}$$

Equation (141) is a single equation for the membrane shape $r$, and can easily be non-dimensionalized with Eqs. (46)–(48). Multiplying the dimensionless equation by $(r^*)^2/4$, and dropping the '$*$' accents for notational simplicity, we find

$$r_{,t}\,+\,SL\,r_{,z}\;=\;\frac{\Gamma}{4}\left(r^2\,-\,r\,+\,r^2 r_{,zz}\right)\,-\,\frac{1}{16}\left(r^2\,-\,\frac{1}{r}\,+\,r_{,zz}\,+\,2r^2 r_{,zzzz}\right)\,. \tag{142}$$

At this point, we seek to express algebraic quantities in Eq. (142) in term of $(r-1)$, namely the deviation from the base radius. To this end, we substitute $r^2 - r = (r-1)+(r-1)^2$ and $r^2 - 1/r = 3(r-1)+(r-1)^2-(r-1)^2/r$ into Eq. (142) and rearrange terms to obtain

$$\begin{aligned} r_{,t}\,+\,SL\,r_{,z}\;=\;&\left(\frac{\Gamma-\Gamma_0}{4}\right)r_{,zz}\,-\,\frac{1}{8}\,r_{,zzzz}\,+\,\left(\frac{\Gamma-\Gamma_c}{4}\right)(r-1)\,+\,\left(\frac{\Gamma-\Gamma_0}{4}\right)(r-1)^2\,+\,\frac{1}{16}\,\frac{(r-1)^2}{r} \\ &+\,\Big[(r-1)^2+2(r-1)\Big]\left(\frac{\Gamma}{4}\,r_{,zz}\,-\,\frac{1}{8}\,r_{,zzzz}\right)\,. \end{aligned} \tag{143}$$

Finally, we once again assume the membrane shape is weakly varying, such that $(r-1)^j * \partial_z^k r$ is negligible relative to $(r-1)^j$ for $k \geq 1$. In this case, Eq. (143) simplifies to

$$r_{,t}\,+\,SL\,r_{,z}\;=\;\left(\frac{\Gamma-\Gamma_0}{4}\right)r_{,zz}\,-\,\frac{1}{8}\,r_{,zzzz}\,+\,\left(\frac{\Gamma-\Gamma_c}{4}\right)(r-1)\,+\,\left(\frac{\Gamma-\Gamma_0}{4}\right)(r-1)^2\,+\,\frac{1}{16}\,\frac{(r-1)^2}{r}\;, \tag{144}$$

which is a single equation for the shape evolution of a perturbed membrane tube. As expected, Eq. (144) simplifies to Eq. (58) when nonlinear terms are neglected, with $\tilde{r} = r - 1$.

While Eq. (144) is indeed a single nonlinear equation for the dynamics of a perturbed lipid membrane tube, solving the equation numerically leads to the same difficulties as those from the linearized case (see discussion in Sec. III.4). We thus make the change of variables presented in Eq. (114), for which Eq. (144) can be written as

$$r_{,T}\,+\,\overline{SL}\,r_{,Z}\;=\;r_{,ZZ}\,-\,\frac{1}{2}\,\frac{(\Gamma-\Gamma_c)}{(\Gamma-\Gamma_0)^2}\,r_{,ZZZZ}\,+\,f(r)\;, \tag{145}$$

where the forcing term $f(r)$ is given by

$$f(r)\;=\;(r-1)\,+\,\left(\frac{\Gamma-\Gamma_0}{\Gamma-\Gamma_c}\right)(r-1)^2\,+\,\left(\frac{\Gamma_0}{\Gamma-\Gamma_c}\right)\frac{(r-1)^2}{r}\;. \tag{146}$$

Equation (145) has the structure of an EFK equation, with the forcing term $f(r)$ plotted for three values of $\Gamma$ in Fig. 6a, and a zoom around $r = 1$ shown in Fig. 6b. Note that in the absence of temporal variations

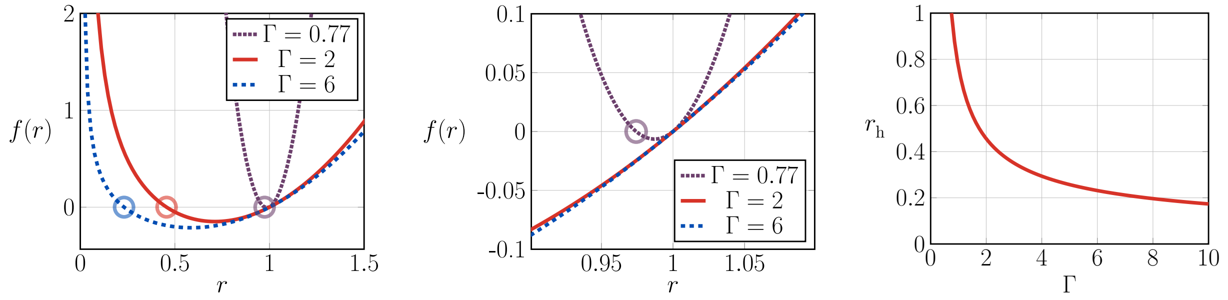


(a) nonlinear forcing (b) nonlinear forcing near $r = 1$ (c) homogeneous radius

Figure 6: (a),(b): Plots of the weakly nonlinear forcing term $f(r)$ in Eq. (146), at three different Föppl–von Kármán numbers: $\Gamma = 0.77$, $\Gamma = 2$, and $\Gamma = 6$. Open circles indicate stable solutions where $f(r) = 0$. Here, (b) shows a zoom of the forcing term near $r = 1$. (c) Plot of the homogeneous radius $r_{\text{h}}$, as a function of the Föppl–von Kármán number, for all unstable $\Gamma > \Gamma_{\text{c}}$.

($r_{,T} = 0$) and spatial gradients ($r_{,Z} = 0$), the evolution equation (145) simplifies to $f(r) = 0$. As shown in Figs. 6a and 6b, the slope of $f(r)$ at $r = 1$ is positive, implying the base solution is unstable. However, in all cases there exists another solution of $f(r) = 0$, denoted the homogeneous radius $r_{\text{h}}$ and given by

$$r_{\text{h}} = 1 + \frac{1}{8\Gamma - 2}\left(3 - 8\Gamma + \sqrt{16\Gamma - 3}\right) . \tag{147}$$

As $f'(r_{\text{h}}) < 0$, a tube of radius $r_{\text{h}}$ is stable. Figure 6c plots the homogeneous radius as a function of the Föppl–von Kármán number, and shows $r_{\text{h}} < 1$ for all $\Gamma > \Gamma_{\text{c}}$. The evolution equation thus predicts that when fronts are propagating along the $z$-axis away from an initially localized perturbation, the thin tube that develops behind the front is of radius $r_{\text{h}}$. Note that Eq. (147) is provided in the discussion below Fig. 4 of the main text, while Eqs. (145) and (146) are presented as Eqs. (5) and (6) in the main text. While the EFK equation (145) provides a simplified description of the dynamics of lipid membrane tubes, it includes only weak nonlinearities and is expected to be quantitatively predictive in limited regimes of mild tube deformations. We now proceed to test the validity of Eq. (145) by comparing its shape predictions to results from simulations of the full nonlinear equations.

## 2. Weakly vs. fully nonlinear simulations

In order to compare our EFK model to direct numerical simulations, we carry out tests at different values of the Föppl–von Kármán number and for three types of shape disturbances: (i) an inward localized perturbation, (ii) an outward localized perturbation, and (iii) a sinusoidal global perturbation. For both the EFK and fully nonlinear simulations, we begin with an unperturbed cylinder of radius $r_0 = 1$, length $\ell_0$, and tension $\lambda_0 = \Gamma$—the latter being in units of $k_{\text{b}}/r_0^2$, with $k_{\text{b}}$ set to unity. Note that in our numerical implementation, we set $\zeta = 1$ as well; all other quantities are then specified by the chosen values of $\Gamma$ and $SL$. In terms of the area parametrization introduced in Sec. I.3 (a), we have $a \in [0, 2\pi r_0 \ell_0]$, where for an unperturbed cylinder $a = 2\pi r_0 z$. At time $t = 0$, we apply a radial perturbation, and then solve for the membrane shape over time. The EFK equation (145) is solved with the finite element solver `FreeFEM` [40], with the fourth-order spatial derivative necessitating two boundary conditions ($r = 1$ and $r_{,z} = 0$) be specified on each end of the spatial domain. For ease in comparison, results from EFK simulations are presented in terms of the unscaled axial position $z$ and time $t$, rather than their scaled counterparts $Z$ and $T$ introduced in Eq. (114). The fully nonlinear equations are solved with an in-house code similar to that described in Ref. [7], which employs the `BVP5C` solver in `MATLAB` to solve the system of first-order ODEs in Eqs. (18)–(25). Eight boundary conditions are prescribed, corresponding to our eight first-order ODEs. In each of the following scenarios, we present the initial radial perturbation, boundary conditions for both simulations, and numerical results.

## (a). Inward localized perturbation

All numerical simulations shown in the main text are initially perturbed with an inward Gaussian. In terms of the axial distance $z = a/(2\pi r_0)$ of the unperturbed tube, the radius at time $t = 0$ is prescribed to be

$$r(z, t = 0) \; = \; r_0 \left[ 1 \, - \, \epsilon \, \exp\left( - \, \frac{(z - \bar{\mu})^2}{2\sigma^2} \right) \right] \, , \tag{148}$$

where the Gaussian is centered at $z = \bar{\mu}$ and has half-width $\sigma = 2r_0$. In Eq. (148) and from now on, $\epsilon = 10^{-3}$ is a small parameter.

## Fully nonlinear simulations

Figures 1(b) and 3 in the main text correspond to a membrane tube with a base flow, for which the eight boundary conditions are given by

$$r(0) \, = \, r_0 \, , \qquad z(0) \, = \, 0 \, , \qquad \lambda(0) \, = \, \lambda_0 \, , \qquad H(0) \, = \, H_0 \, , \qquad u(0) \, = \, u_0 \, , \qquad w(0) \, = \, 0 \, ,$$
$$\varphi(A) \, = \, \varphi_0 \, , \qquad L(A) \, = \, 0 \, , \tag{149}$$

where for notational convenience we introduce we introduce the following quantities to correspond to an unperturbed tube:

$$H_0 \; := \; \frac{-1}{2r_0} \, , \qquad \varphi_0 \; := \; \frac{\pi}{2} \, , \qquad u_0 \; := \; 2\pi r_0 SL \, , \qquad \text{and} \qquad A \; := \; 2\pi r_0 \ell_0 \, . \tag{150}$$

In the aforementioned simulations, we choose for the Gaussian to be centered at $\bar{\mu} = \ell_0/4$, where $\ell_0$ is chosen to be large enough that tube dynamics are not affected by the finite size of the system. Just as Figs. 1(b) and 3 in the main text showed numerical results for $\Gamma = 6$ and $SL/SL_{\text{ac}} = \{0.25, 2\}$, here we present one additional result corresponding to the absolute-to-convective transition ($SL/SL_{\text{ac}} = 1$) for $\Gamma = 6$, as shown in Fig. 7. Note that Fig. 7b reveals the velocity of the trailing front is zero, as predicted by the linear theory $(123)_2$—thus confirming the system is at the threshold between absolutely unstable and convectively unstable tubes.

The main text also presents simulations of a membrane tube with no base flow. Such a tube is symmetric about the center of the Gaussian perturbation, which we choose to be at $\bar{\mu} = 0$. Accordingly, only half the

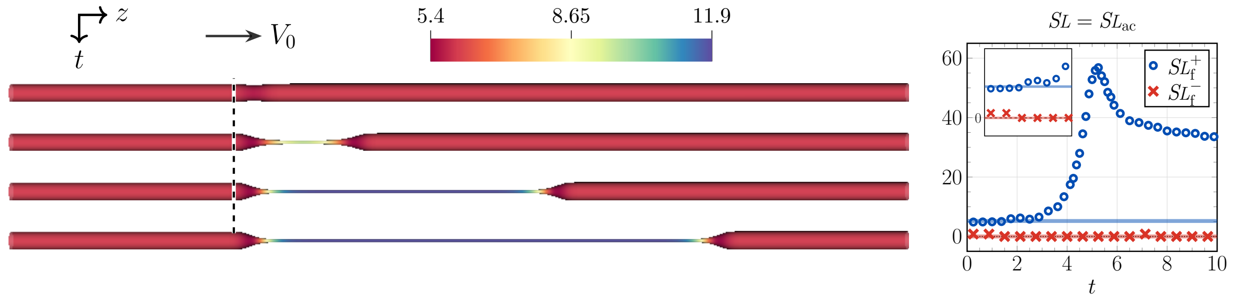


(a) membrane shapes over time

(b) front velocities

Figure 7: Results from numerical simulation of a membrane tube, with $\Gamma = 6$ and $SL = SL_{\text{ac}}$. (a) Snapshots of the membrane shape over time, with the initially localized perturbation at the vertical dashed line. Here, the $z$-axis is scaled by a factor of $^1\!/_4$, as opposed to Fig. 1(b) of the main text, in which the $z$-axis is scaled by a factor of $^1\!/_{40}$. (b) Plot of the leading and trailing front velocities, similar to Fig. 3 in the main text. Note the trailing front velocity is zero, as expected for a system at the absolute-to-convective transition.

domain is simulated, for which the boundary conditions are given by

$$\begin{aligned} z(0) &= 0 \,, & \varphi(0) &= \varphi_0 \,, & u(0) &= 0 \,, & L(0) &= 0 \,, \\ \varphi(A) &= \varphi_0 \,, & \lambda(A) &= \lambda_0 \,, & w(A) &= 0 \,, & L(A) &= 0 \,. \end{aligned} \tag{151}$$

All simulation results of a localized inward perturbation to a tube with no base flow are shown in Fig. 4 of the main text, which highlighted how the front is monotonic when $\Gamma \in \Omega_{\rm A}$ and oscillatory when $\Gamma \in \Omega_{\rm B}$.

As it turns out, the oscillating fronts arising when $\Gamma \in \Omega_{\rm B}$ lead to numerical difficulties: the front sheds oscillatory modes, some of which reflect off the right boundary and contaminate the computational domain. To prevent such reflections, we follow past numerical developments in open flow systems [41] and introduce a so-called sponge zone to dampen would-be reflected waves. In particular, when simulating a tube with area $A = 2\pi r_0 \ell_0$, we extend our computational domain to have area $1.5A$; in the final third of the domain we also increase the numerical value of the intramembrane viscosity $\zeta$ to dampen reflected oscillatory modes. Denoting $\zeta_{\rm sim}$ as the value of the parameter used in numerical simulations, we have

$$\frac{\zeta_{\rm sim}}{\zeta} = \begin{cases} 1 & 0 \le a \le A \,, \\ 1 + 2\left[1 + \exp\left(\dfrac{\delta_{\rm r}}{a - A} - \dfrac{\delta_{\rm r}}{a + \delta_{\rm r} - A}\right)\right]^{-1} & A < a \le A + \delta_{\rm r} \\ 3 & a > A + \delta_{\rm r} \,, \end{cases} \tag{152}$$

where $\delta_{\rm r}$ is the length of the region over which the viscosity ramps up—here set to $0.25A$. We note that the size of the sponge zone, the ramp up length, and the maximum value of $\zeta_{\rm sim}$ were varied until oscillatory modes were no longer reflected into the domain, and are valid only for the specific problem at hand. As a validation test, we applied a sponge zone to simulations in which $\Gamma \in \Omega_{\rm A}$, and found the numerical results were completely unchanged. The results presented in Figs. 1, 3, and 4 of the main text, as well as Fig. 7, conclude all fully nonlinear simulations corresponding to spatially localized, inward perturbations.

## EFK equation simulations

The dashed lines in Fig. 4 of the main text are numerical solutions of the weakly nonlinear EFK equation (145), with no base flow ($SL = 0$). In this case, we simulate the domain $z \in [-\ell_0, \ell_0]$, with the symmetric boundary conditions

$$r(-\ell_0) = r_0 \,, \qquad r_{,z}(-\ell_0) = 0 \,, \qquad r(\ell_0) = r_0 \,, \qquad r_{,z}(\ell_0) = 0 \,, \tag{153}$$

where as before we choose $r_0 = 1$. Here, we provide additional results from simulations with a base flow, at $\Gamma = 6$, as shown in Fig. 8. The pulled fronts move at a speed predicted by the linear theory, and in all cases the thin tube saturates at the radius $r = r_{\rm h}(\Gamma = 6) \approx 0.23$.

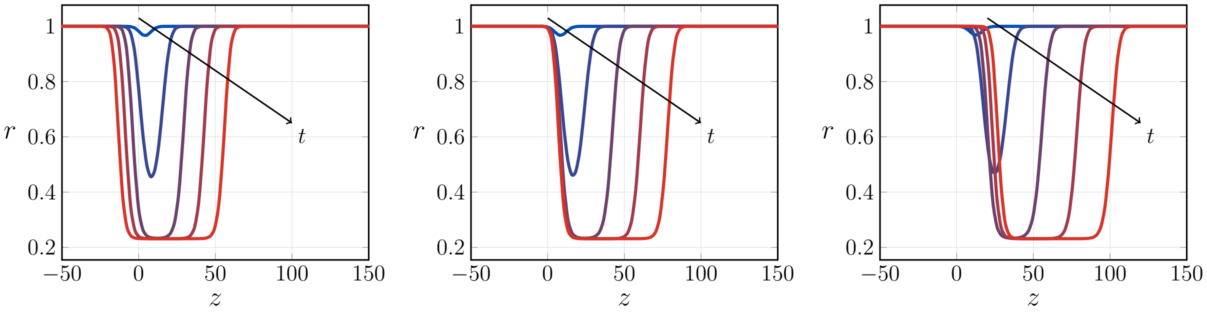


(a) $SL = 0.5\,SL_{\rm ac}$ (b) $SL = SL_{\rm ac}$ (c) $SL = 1.5\,SL_{\rm ac}$

Figure 8: Snapshots from simulations of the EFK equation (145), at three different base flow speeds with $\Gamma = 6$. In all cases, the initial perturbation is at $z = 0$, snapshots are separated by $\approx 3\tau$, and the leading front travels to the right. The trailing front (a) travels to the left when $SL < SL_{\rm ac}$, (b) remains stationary when $SL = SL_{\rm ac}$, and (c) travels to the right when $SL > SL_{\rm ac}$.

As discussed in the main text, the EFK equation predicts propagating fronts when $\Gamma \in \Omega_{\mathrm{A}}$ and fails when $\Gamma \in \Omega_{\mathrm{B}}$—as explained in the following subsection. Moreover, the EFK equation agrees quantitatively well with fully nonlinear simulations for $\Gamma \in [\Gamma_{\mathrm{c}}, \Gamma_1]$, where our weakly nonlinear assumptions are most accurate and membrane shape perturbations remain small. Finally, we found that in all cases the MSC predicts the leading and trailing front velocities of the EFK equation, only the latter of which agrees with fully nonlinear simulations. We leave a more detailed analysis of the front velocities to a future study.

## (b). Outward localized perturbation

We next consider a local, outward perturbation, for which the initial radius is given by [cf. Eq. (148)]

$$r(z, t = 0) \;=\; r_0 \left[ 1 \,+\, \epsilon \, \exp\left( -\,\frac{z^2}{2\sigma^2} \right) \right] \,, \tag{154}$$

where as before $r_0 = 1$, $\sigma = 2r_0$, and $\epsilon = 10^{-3}$. For this type of perturbation, we consider initially static tubes ($SL = 0$), for which the system is symmetric. We first discuss why the evolution equation is unable to describe the long-time dynamics of such a perturbation, and then present the fully nonlinear simulations—along with a simplified analytical description of their long-time behavior.

### EFK equation simulations and finite time blow-up

When an unstable membrane tube is perturbed slightly outwards, the small disturbance will initially grow exponentially according to the linear theory. Eventually, nonlinear effects will become significant, and in the case of the EFK equation (145) the nonlinear forcing term $f(r)$ no longer causes the instability to saturate—rather, it continuously amplifies the perturbation. The instability amplification eventually leads to a finite time blow-up, as shown in Fig. 9. We now characterize the behavior of our EFK model, expressed in terms of the unscaled variables $z$ and $t$ (144), as it approaches the blow-up time $t_{\mathrm{c}}$. To this end, note that for very large perturbations ($r - 1 \gg 0$), the nonlinear dynamics can be approximated by

$$r_{,t} \;\approx\; \left( \frac{\Gamma - \Gamma_0}{4} \right) (r-1)^2 \;. \tag{155}$$

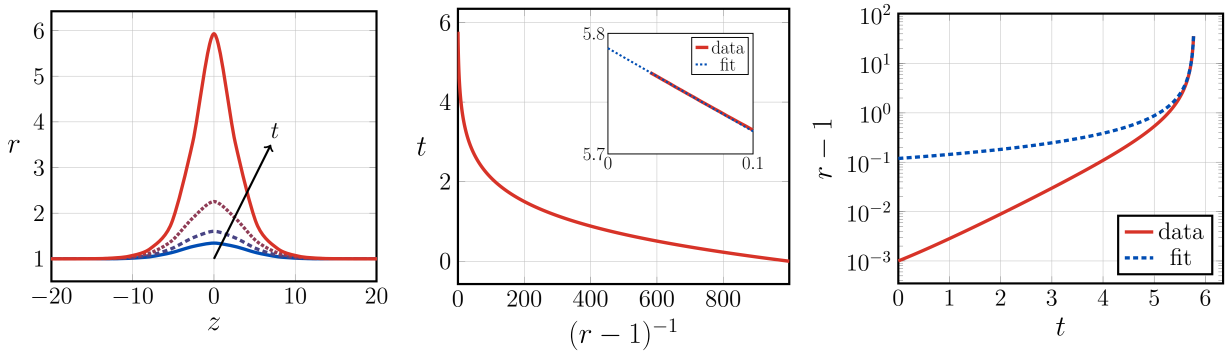


(a) membrane shape over time (b) data fit near blow-up (c) agreement at late times

Figure 9: Finite time blow-up of the EFK equation. (a) Evolution of the membrane shape. Snapshots are separated by the same time interval, showing how the maximum radius rapidly increases once deformations become large. (b) A plot of $T$ vs. $1/(r-1)$ is used to calculate the blow-up time $T_{\mathrm{c}}$ and the proportionality constant $\alpha$, as described in the main text. Here, $r$ refers to the maximum tube radius, which occurs at $Z = 0$. (c) A plot the maximum radius as a function of time reveals the prediction of Eq. (157) agrees with simulation results at late times.

We integrate Eq. (155) from a given time $t$ up to the blow-up time $t_\mathrm{c}$, at which point the radius becomes infinite, and write

$$\int_r^\infty \frac{\mathrm{d}r}{(r-1)^2} \approx \int_t^{t_\mathrm{c}} \left(\frac{\Gamma - \Gamma_0}{4}\right) \mathrm{d}t \; . \tag{156}$$

Equation (156) indicates the long-time behavior of the tube radius is given by

$$r - 1 \approx \left[\alpha\left(t_\mathrm{c} - t\right)\right]^{-1} \quad \text{as} \quad t \to t_\mathrm{c} \; , \tag{157}$$

where $\alpha$ is a constant of proportionality that is predicted to be $(\Gamma - \Gamma_0)/4$. To determine $\alpha$ and $t_\mathrm{c}$ from the simulation data, we recognize Eq. (157) can be written as $t = t_\mathrm{c} - [\alpha(r-1)]^{-1}$. Thus, by plotting $t$ as a function of $1/(r-1)$ as in Fig. 9b, we fit a straight line to data near the blow-up and find $t_\mathrm{c} = 5.79$ and $\alpha = 1.45$—the latter being close to the predicted value of 1.44 at $\Gamma = 6$. Note that while our analysis in this section was focused on an initially local disturbance, the blow-up phenomenon described here applies to any outward perturbation in the EFK model. As a result, the EFK equation is unable to describe an inward perturbation when $\Gamma \in \Omega_\mathrm{B}$: the oscillating front leads to both inward and outward shape variations, and the latter will eventually be amplified and singularly blow up.

## Fully nonlinear simulations and simplified model for late-time pearl growth

Given the blow-up of the EFK equation, we now use the fully nonlinear equations to study the response of membrane tubes to an outward perturbation. Only systems with no base flow are considered. Accordingly, the system is symmetric—allowing us to simulate only half of the domain. In this case, the eight boundary conditions are given by

$$\begin{aligned} z(0) &= 0 \; , & \varphi(0) &= \varphi_0 \; , & u(0) &= 0 \; , & L(0) &= 0 \; , \\ r(A) &= r_0 \; , & H(A) &= H_0 \; , & w(A) &= 0 \; , & L(A) &= 0 \; . \end{aligned} \tag{158}$$

As shown in Fig. 10a for the case when $\Gamma = 6$, the initial outward perturbation continues to draw in lipids and eventually forms a pearl; the dashed green lines are spherical cross-sections provided for comparison. The pearl grows over time, and is connected to the unperturbed cylinder by a narrow transition region. In what follows, we provide a simple explanation for the observed long-time membrane response to a local outward perturbation. To this end, we analyze the general axisymmetric equations (13)–(15) in the spherical, cylindrical, and transition regions, in which all quantities are respectively labeled with a subscript 's', 'c', or 't'. Thus, for example, $\lambda_\mathrm{c}$ is the surface tension in the cylindrical region. Note that since we have so far used the symbol $r$ to denote the distance from the axis of rotation, here we use the symbol $\rho_\mathrm{s}$ for the sphere radius. In all of our analysis, out-of-plane viscous forces are neglected for simplicity.

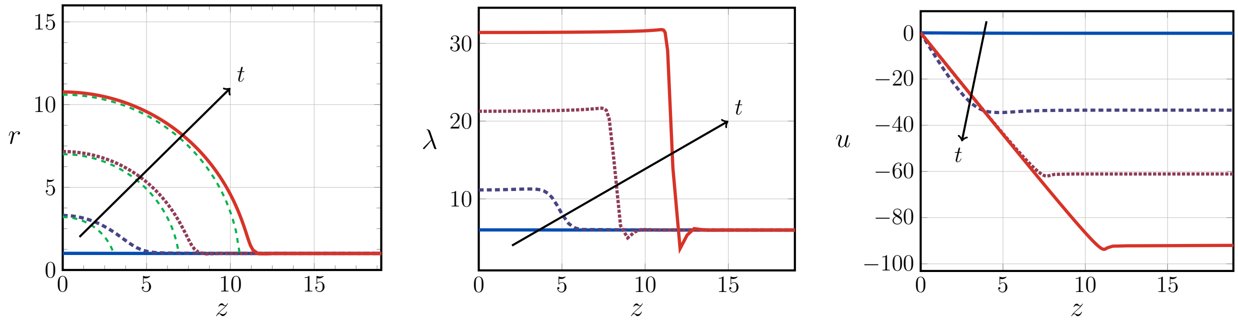


(a) radius $r(z,t)$ (b) surface tension $\lambda(z,t)$ (c) in-plane velocity $u(z,t)$

Figure 10: Snapshots of the radius (a), surface tension (b), and inplane velocity (c) at times $t = 3$, $t = 8$, $t = 13$, and $t = 18$, all for an outward Gaussian perturbation with $\Gamma = 6$. Dashed green lines in (a) show the cross-section of a perfect sphere.

The pearled morphology is approximated as a sphere of radius $\rho_\mathrm{s} = \rho_\mathrm{s}(t)$, for which the corresponding mean and Gaussian curvatures are given by $H_\mathrm{s} = -1/\rho_\mathrm{s}$ and $K_\mathrm{s} = 1/\rho_\mathrm{s}^2$, respectively. Additionally, kinematics require for the normal velocity to satisfy $v_\mathrm{s} = \mathrm{d}\rho_\mathrm{s}/\mathrm{d}t$ in the spherical region. Taking the spatial derivative of the continuity equation (13), recalling spatial derivatives with respect to the area parametrization are denoted as $(\,\cdot\,)'$, and recognizing that both $v_\mathrm{s}' = 0$ and $H_\mathrm{s}' = 0$ due to our assumption of a spherical geometry, we find $u_\mathrm{s}'' = 0$. Additionally, with our assumption that viscous forces are negligible in the normal direction, the shape equation (15) simplifies to

$$p \;=\; \frac{2\lambda_\mathrm{s}}{\rho_\mathrm{s}} \;. \tag{159}$$

Taking the spatial derivative of both sides of Eq. (159) and recalling that the pressure $p$ is everywhere constant reveals $\lambda_\mathrm{s}' = 0$, and shows that the spherical surface tension does not vary in space and is given by

$$\lambda_\mathrm{s}(t) \;=\; \frac{1}{2}\, p\, \rho_\mathrm{s}(t) \;. \tag{160}$$

Next, consider the cylindrical region, whose shape is unchanged as the spherical pearl grows. The cylinder radius $r_\mathrm{c} = r_0$ is constant, for which $H_\mathrm{c} = -1/(2r_0)$, $K_\mathrm{c} = 0$, and $v_\mathrm{c} = 0$. The continuity equation (13) then requires $u_\mathrm{c}' = 0$, for which $u_\mathrm{c} = u_\mathrm{c}(t)$—as confirmed by the unchanging value of $u$ in the cylindrical regions of Fig. 10c. The shape equation (15) then simplifies to

$$p \;=\; \lambda_\mathrm{c} r_\mathrm{c} \;-\; \frac{k_\mathrm{b}}{4r_\mathrm{c}^2} \;, \tag{161}$$

confirming that $\lambda_\mathrm{c}$ is constant in the unperturbed cylinder.

To relate quantities in the spherical and cylindrical regions, we investigate the narrow transition zone between them. In this region, we observe from Fig. 10 that $u_\mathrm{t} \approx u_\mathrm{c}$ and $r_\mathrm{t} \approx r_0$, and we make the additional assumption that the normal velocity in the transition region $v_\mathrm{t} \approx 0$. At this point, we seek to integrate the in-plane equation (14) over the transition region. To do so, we require the values of the area parametrization $a$ at the start and end of this region. Consider the latest snapshot in Fig. 10a: we have $a_\mathrm{s} \approx 2\pi\rho_\mathrm{s}^2$ when $z \approx 11$, where $a_\mathrm{s}$ denotes the total surface area between $z = 0$ and the edge of the pearl. It is useful to note that at this location, the parametric angle $\varphi_\mathrm{s} \approx \pi$ (see Fig. 1 for a depiction of $\varphi$). We similarly denote $a_\mathrm{c}$ to be the value of the area parametrization at the start of the cylindrical region, for which the corresponding parametric angle $\varphi_\mathrm{c} \approx \pi/2$. With these observations, we integrate the in-plane equation (14) to obtain

$$\int_{a_\mathrm{s}}^{a_\mathrm{c}} \lambda' \;\mathrm{d}a \;=\; -\frac{\zeta u_\mathrm{c}}{\pi r_0^2} \int_{a_\mathrm{s}}^{a_\mathrm{c}} \sin\varphi\,\varphi' \;\mathrm{d}a \;=\; -\frac{\zeta u_\mathrm{c}}{\pi r_0^2} \int_{\varphi_\mathrm{s}}^{\varphi_\mathrm{c}} \sin\varphi \;\mathrm{d}\varphi \;, \tag{162}$$

where $\varphi'\mathrm{d}a = \mathrm{d}\varphi$. Equation (162) then yields

$$\lambda_\mathrm{s}(t) \;=\; \lambda_\mathrm{c} \;-\; \frac{\zeta u_\mathrm{c}}{\pi r_0^2} \;, \tag{163}$$

which upon substitution into the spherical shape equation (159) reveals

$$\frac{1}{2}\, p\rho_\mathrm{s}(t) \;=\; \lambda_\mathrm{c} \;-\; \frac{\zeta u_\mathrm{c}}{\pi r_0^2} \;. \tag{164}$$

At this point, we seek to express $u_\mathrm{c}(t)$ in terms of $r_\mathrm{s}(t)$. To this end, we integrate the continuity equation (13) over half of the sphere, from $a = 0$ to $a_\mathrm{s} = 2\pi\rho_\mathrm{s}^2$. By recognizing $v_\mathrm{s}$ and $H_\mathrm{s}$ do not spatially vary over the spherical region, we find

$$\int_0^{a_\mathrm{s}} u' \;\mathrm{d}a \;=\; -\frac{2v_\mathrm{s}}{\rho_\mathrm{s}} \int_0^{a_\mathrm{s}} \mathrm{d}a \;, \qquad \text{such that} \qquad u(a_\mathrm{s}) \;-\; u(0) \;=\; -4\pi v_\mathrm{s}\rho_\mathrm{s} \;. \tag{165}$$

To simplify Eq. (165), we recognize $u(0) = 0$ from our boundary conditions (158), $v_\mathrm{s} = \mathrm{d}r_\mathrm{s}/\mathrm{d}t$ according to our kinematic requirements, and $u(a_\mathrm{s}) \approx u_\mathrm{t} \approx u_\mathrm{c}$ (see Fig. 10c). Thus, the in-plane velocity in the cylindrical region is related to the sphere radius by

$$u_\mathrm{c} \;=\; -4\pi\rho_\mathrm{s}\frac{\mathrm{d}\rho_\mathrm{s}}{\mathrm{d}t} \;=\; -\frac{\mathrm{d}}{\mathrm{d}t}\big(2\pi\rho_\mathrm{s}^2\big) \;, \tag{166}$$

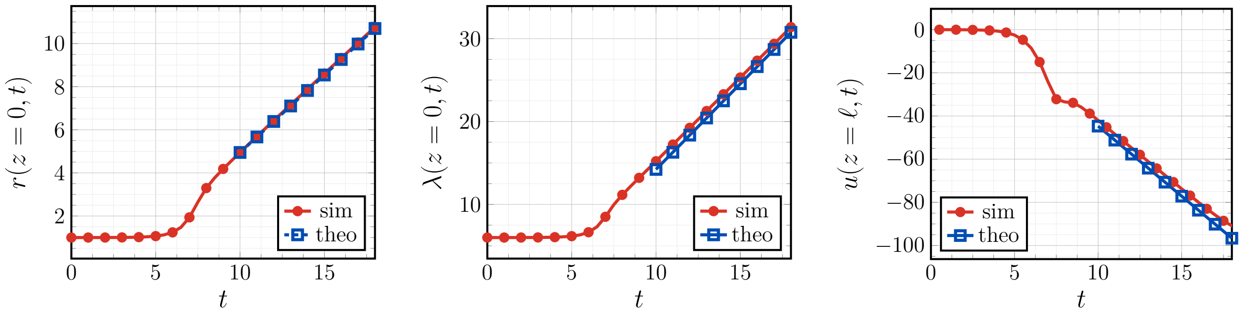


(a) radius at $z = 0$ (b) surface tension at $z = 0$ (c) in-plane velocity at $z = \ell_0$

Figure 11: Comparison of simulation results and theoretical calculations of the maximum radius (a), maximum surface tension (b), and minimum velocity (c). We use the maximum radius at $t = 10$ as a parameter in the model, but otherwise there are no fitting parameters.

showing that the in-plane velocity in the cylindrical region is supplying the additional lipids required for the sphere to grow. Substituting Eq. (166) into Eq. (164) yields a single differential equation for the sphere radius, written as

$$\frac{\mathrm{d}\rho_{\mathrm{s}}}{\mathrm{d}t} = \frac{r_0^2}{4\zeta}\left(\frac{p}{2} - \frac{\lambda_{\mathrm{c}}}{\rho_{\mathrm{s}}}\right) . \tag{167}$$

In obtaining Eq. (167), we assumed the deformed membrane morphology was approximately a sphere connected to a cylinder. If the sphere radius is large at some arbitrary time $t_1$, then the second term in parenthesis in Eq. (167) is negligible and we find a simple expression for the evolution of the sphere radius, given by

$$r_{\mathrm{s}}(t) = r_{\mathrm{s}}(t_1) + \frac{r_0^2}{4\zeta}\frac{p}{2}\left(t - t_1\right) . \tag{168}$$

In dimensionless form, Eq. (168) is written as

$$r_{\mathrm{s}}^*(t) = r_{\mathrm{s}}^*(t_1^*) + \frac{1}{8}\left(\Gamma - \Gamma_0\right)\left(t^* - t_1^*\right) . \tag{169}$$

With an expression for the sphere radius in Eq. (169), we can obtain $\lambda_{\mathrm{s}}$ via the shape equation (159), and subsequently the cylindrical in-plane velocity with Eq. (164). In dimensionless form, these two quantities can be written as

$$\lambda_{\mathrm{s}}^*(t) = \frac{1}{2}\left(\Gamma - \Gamma_0\right) r_{\mathrm{s}}^*(t^*) \tag{170}$$

and

$$u_{\mathrm{c}}^* = -\frac{\pi}{2}\left(\Gamma - \Gamma_{\mathrm{c}}\right) r_{\mathrm{s}}^*(t^*) . \tag{171}$$

Figure 11 shows that the approximate solutions given in Eqs. (169)–(171) are in good agreement with the fully nonlinear simulations for the case of an outward Gaussian perturbation at $\Gamma = 6$, where the only fitting parameter is a single value of the sphere radius at an arbitrarily chosen time. Thus, our analysis shows that at long times, an initially outward local perturbation results in an expanding spherical pearl in contact with the initial cylinder.

## (c). Global perturbation

The final class of initial disturbances we consider is a long-wavelength, sinusoidal perturbation along the entire domain, for which the initial membrane shape is given by

$$r(z, t = 0) = r_0\left[1 - \epsilon\cos\left(\frac{3z}{2\ell_0}\right)\right] . \tag{172}$$

As discussed previously, the presence of initial outward bulges leads to a finite time blow-up of the EFK equation (145). Accordingly, the EFK equation will again not be able to reveal membrane morphologies at long times. In what follows, we first report the results from fully nonlinear simulations. We then once again provide an approximate analytical description of the nonlinear shapes observed at late times.

### Fully nonlinear simulations and simplified model for late-time pearls and tubes

For global perturbations of the form in Eq. (172), we prescribe the boundary conditions

$$\begin{aligned} z(0) &= 0\,, \qquad \varphi(0) = \varphi_0\,, \qquad u(0) = 0\,, \qquad L(0) = 0\,, \\ z(A) &= \ell_0\,, \qquad \varphi(A) = \varphi_0\,, \qquad u(A) = 0\,, \qquad L(A) = 0\,. \end{aligned} \tag{173}$$

Results from our numerical simulations at $\Gamma = 0.77$, 2, and 6 are respectively shown in Figs. 12–14. In all cases, a sinusoidal shape remains at early times, and a 'beads-on-a-string' configuration is seen at late times. We note that as $\Gamma$ is increased, the beaded morphology more closely resembles a sphere, with the surface tension being roughly constant in both the spherical and thin cylindrical regions. The long-time pearled shapes obtained in Figs. 12–14 are qualitatively similar to those seen in experimental investigations of unstable lipid membrane tubes [13, 42].

As in the case of a localized outward perturbation, we now seek to provide a simple analytical explanation of the observed beads-on-a-string morphology at late times. We consider a portion of the tube corresponding to a single wavelength of the initial perturbation, which in this case is of length $\bar{\ell} := 2\ell_0/3$. At long times, this portion of the membrane is approximated as a spherical pearl of radius $\rho_{\mathrm{s}}$ connected to a thin cylinder of length $\ell_{\mathrm{c}}$ and radius $r_{\mathrm{c}}$, as shown in Fig. 15. Importantly, as the shape evolves, both the length and area of the membrane remain constant—which respectively require

$$\bar{\ell} = \ell_{\mathrm{c}} + 2\sqrt{\rho_{\mathrm{s}}^2 - r_{\mathrm{c}}^2} \qquad \text{and} \qquad 2\pi r_0 \bar{\ell} = 4\pi\rho_{\mathrm{s}}\sqrt{\rho_{\mathrm{s}}^2 - r_{\mathrm{c}}^2} + 2\pi r_{\mathrm{c}}\ell_{\mathrm{c}}\,. \tag{174}$$

We thus have two equations for the three unknowns $\rho_{\mathrm{s}}$, $r_{\mathrm{c}}$, and $\ell_{\mathrm{c}}$. By assuming the thin tube radius is equal to the homogeneous radius $r_{\mathrm{h}}$ obtained in the analysis of the evolution equation (147), i.e. $r_{\mathrm{c}} = r_{\mathrm{h}}$,

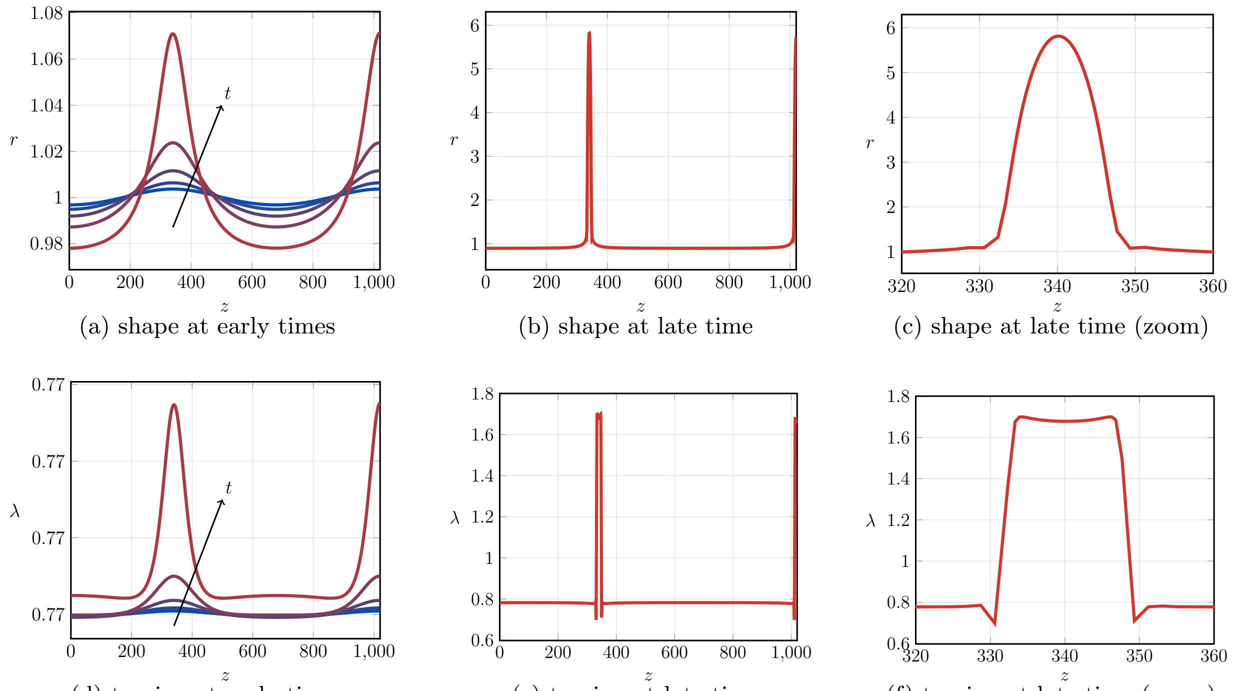


(a) shape at early times (b) shape at late time (c) shape at late time (zoom)

(d) tension at early times (e) tension at late time (f) tension at late time (zoom)

Figure 12: Numerical results from a global sinusoidal shape perturbation, with $\Gamma = 0.77$.

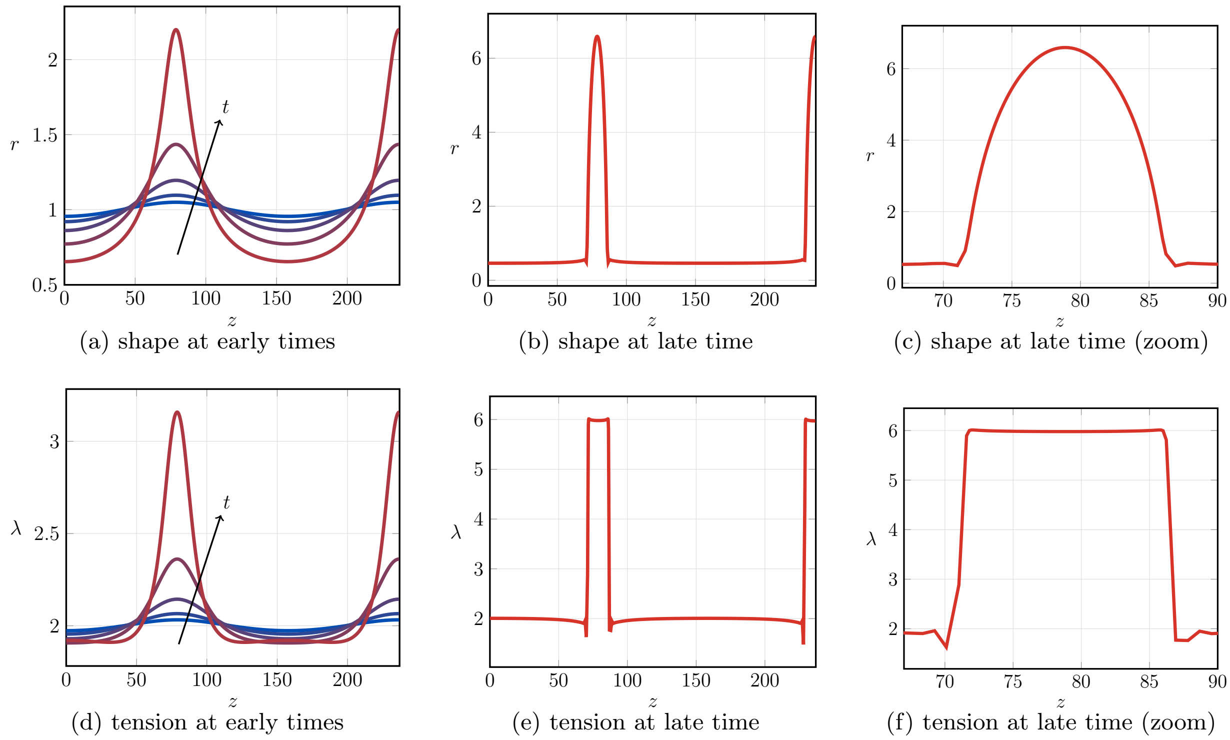


Figure 13: Numerical results from a global sinusoidal shape perturbation, with $\Gamma = 2$.

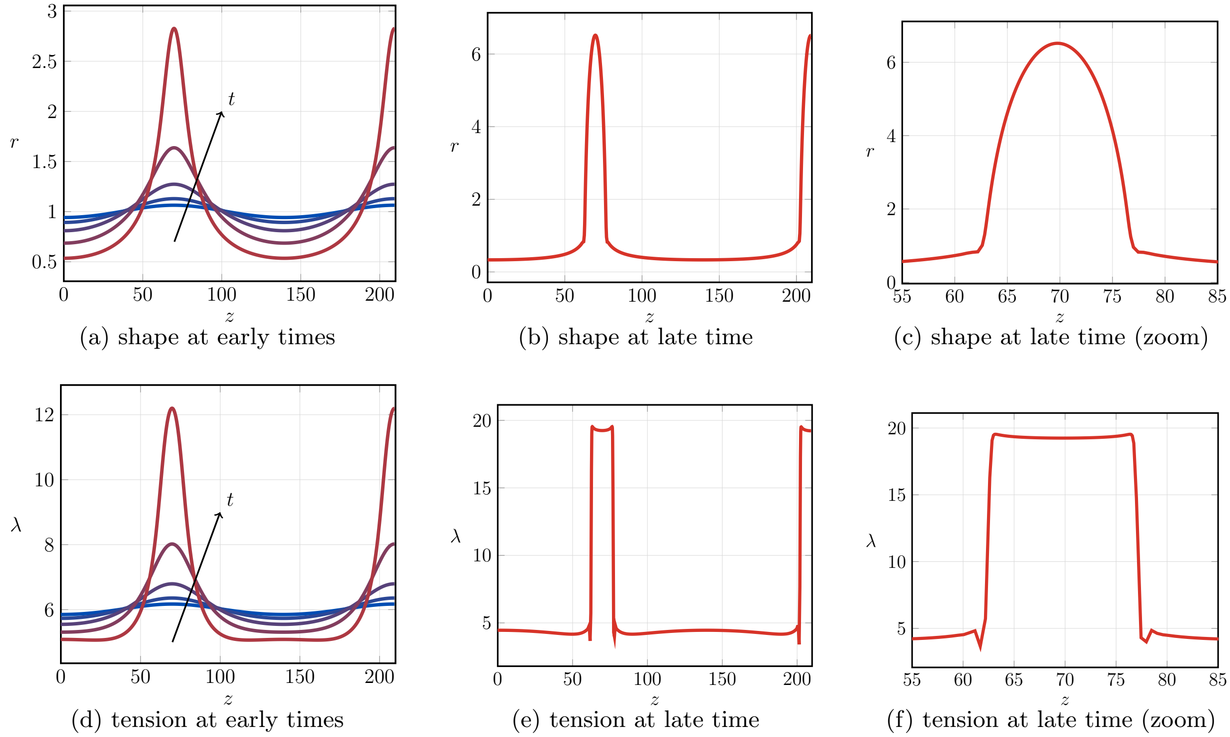


Figure 14: Numerical results from a global sinusoidal shape perturbation, with $\Gamma = 6$.

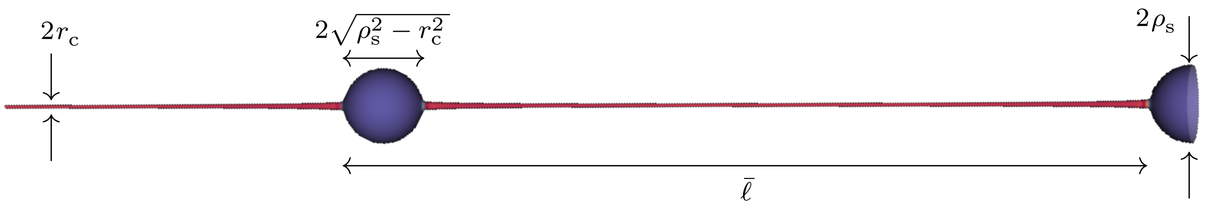


Figure 15: Snapshot of a direct simulation of the pearling instability of a membrane tube initially subjected to a sinusoidal perturbation at $\Gamma = 6$. The computed 'beads-on-a-string' morphology can be approximated by a succession of spherical pearls and cylindrical tubes with dimensions as shown. Note that the axial and radial directions have the same scale here.

we obtain a single equation that can be solved for the sphere radius, namely

$$2\left(\rho_s - r_h\right)\sqrt{\rho_s^2 - r_h^2} = \left(r_0 - r_h\right)\bar{\ell}\,. \tag{175}$$

The value of $\rho_s$ from Eq. (175) is compared to simulation results, for three values of $\Gamma$, in Table 2. Though the agreement is only qualitative, both our simulations and analytical calculations reveal that global perturbations to an unstable membrane tube do indeed yield a 'beads-on-a-string' morphology.

## 3. Final observations

In this section, we investigated how an unstable membrane tube responds to local inward and outward perturbations, as well as a global sinusoidal disturbance. Three characteristic results are shown in Fig. 16. In the case of a global perturbation (Fig. 15, top of Fig. 16), the tube forms a characteristic 'beads on a string' structure, which we found could be reasonably approximated as a set of spherical pearls connected by narrow cylindrical tubes. As discussed in detail in the main text, when a tube is locally perturbed inward (Fig. 16, middle), a thin tube develops in the wake of two propagating fronts. Finally, in response to an initially local outward perturbation, the membrane forms a single sphere connected to the neighboring, unpertubed cylinder—with the long-time morphologies accurately described by a simple model.

| $\Gamma$ | $\bar{\ell}$ | $r_h$ | $\rho_s^{approx}$ | $r_c^{sim}$ | $\rho_s^{sim}$ | $r_c^{error}$ | $\rho_s^{error}$ |
|---|---|---|---|---|---|---|---|
| 0.77 | 680 | 0.97 | 3.54 | 0.89 | 6.00 | 9% | 41% |
| 2 | 158 | 0.46 | 6.79 | 0.46 | 6.60 | 0.4% | 2% |
| 6 | 140 | 0.23 | 7.44 | 0.32 | 6.67 | 28% | 12% |

Table 2: Evaluation of our simple analytical description of the long-time membrane response to a global sinusoidal perturbation (172), for three values of the Föppl–von Kármán number. The value of $\bar{\ell}$ is prescribed by our initial perturbation. We choose for the rescaled axial position $Z \in [0, 200]$, such that [see Eq. (114)] $\ell_0 = 200[(\Gamma - \Gamma_0)/(\Gamma - \Gamma_c)]^{1/2}$ and $\bar{\ell} = 2\ell_0/3$. Values of $r_h$ and $\rho_s^{approx}$ are calculated with Eqs. (147) and (175), respectively; corresponding values from numerical simulations are presented as well. We find the case of $\Gamma = 2$ is best predicted by our approximate model.

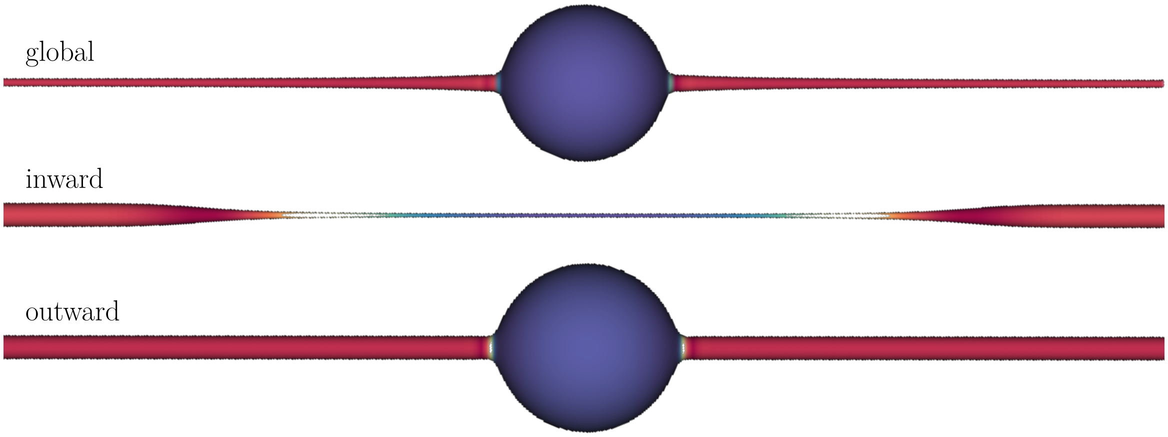


Figure 16: Three-dimensional representations of membrane morphologies resulting from global (top), locally inward (middle), and locally outward (bottom) initial perturbations. In all cases, the radial and axial scales are identical; moreover, all simulations are for $\Gamma = 6$. The results in this figure are not new, but are purely meant to realistically portray the observed membrane shapes.

# References


[1] Sahu, A., Glisman, A., Tchoufag, J. & Mandadapu, K. K. Geometry and dynamics of lipid membranes: The Scriven–Love number. *Phys. Rev. E* **101**, 052401 (2020).

[2] Sahu, A., Sauer, R. A. & Mandadapu, K. K. Irreversible thermodynamics of curved lipid membranes. *Phys. Rev. E* **96**, 042409 (2017).

[3] Evans, E. A. & Skalak, R. *Mechanics and Thermodynamics of Biomembranes* (CRC Press, Boca Raton, Fl., 1980).

[4] Waxman, A. M. Dynamics of a couple-stress fluid membrane. *Studies Appl. Math.* **70**, 63–86 (1984).

[5] Edwards, D. A., Brenner, H. & Wasan, D. *Interfacial Transport Processes and Rheology*. Butterworth-Heinemann Series in Chemical Engineering (Boston: Butterworth-Heinemann, 1991).

[6] Agrawal, A. & Steigmann, D. J. Modeling protein-mediated morphology in biomembranes. *Biomech. Model. Mechan.* **8**, 371–379 (2008).

[7] Omar, Y. A. D., Sahu, A., Sauer, R. A. & Mandadapu, K. K. Non-axisymmetric shapes of biological membranes from locally induced curvature. *Biophys. J.* (2020).

[8] Narsimhan, V., Spann, A. & Shaqfeh, E. Pearling, wrinkling, and buckling of vesicles in elongational flows. *J. Fluid Mech.* **777**, 1–26 (2015).

[9] Chandrasekhar, S. *Hydrodynamic and Hydromagnetic Stability* (Clarendon Press, 2013).

[10] Bar-Ziv, R. & Moses, E. Instability and "pearling" states produced in tubular membranes by competition of curvature and tension. *Phys. Rev. Lett.* **73**, 1392–1395 (1994).

[11] Goldstein, R. E., Nelson, P., Powers, T. & Seifert, U. Front propagation in the pearling instability of tubular vesicles. *J. Phys. II* **6**, 767–796 (1996).

[12] Boedec, G., Jaeger, M. & Leonetti, M. Pearling instability of a cylindrical vesicle. *J. Fluid Mech.* **743**, 262–279 (2014).

[13] Datar, A. *et al.* The roles of microtubules and membrane tension in axonal beading, retraction, and atrophy. *Biophys. J.* **117**, 880–891 (2019).

[14] Bers, A. & Briggs, R. J. Criteria for determining absolute instability and distinguishing between amplifying and evanescent waves. *Bull. Am. Phys. Soc.* **9**, 304 (1963).

[15] Briggs, R. J. *Electron-Stream Interactions with Plasmas* (MIT Press, 1964).

[16] Moser, F. Convective and absolute instability of the positive column with longitudinal magnetic field. *Plasma Physics* **17**, 821–840 (1975).

[17] Merkine, L.-O. Convective and absolute instability of baroclinic eddies. *Geophys. Astro. Fluid* **9**, 129–157 (1977).

[18] Pierrehumbert, R. T. Local and global baroclinic instability of zonally varying flow. *J. Atmos. Sci.* **41**, 2141 (1984).

[19] Huerre, P. & Monkewitz, P. A. Local and global instabilities in spatially developing flows. *Annu. Rev. Fluid Mech.* **22**, 473–537 (1990).

[20] Huerre, P. & Rossi, M. *Hydrodynamic instabilities in open flows*, 81–294 (Cambridge University Press, 1998).

[21] Powers, T. R., Zhang, D., Goldstein, R. E. & Stone, H. A. Propagation of a topological transition: The Rayleigh instability. *Phys. Fluids* **10**, 1052–1057 (1998).

[22] Duprat, C., Ruyer-Quil, C., Kalliadasis, S. & Giorgiutti-Dauphiné, F. Absolute and convective instabilities of a viscous film flowing down a vertical fiber. *Phys. Rev. Lett.* **98**, 244502 (2007).

[23] Scheid, B., Kofman, N. & Rohlfs, W. Critical inclination for absolute/convective instability transition in inverted falling films. *Phys. Fluids* **28**, 044107 (2016).

[24] Charru, F. *Hydrodynamics Instability* (Cambridge University Press, 2011).

[25] Eggers, J. & Villermaux, E. Physics of liquid jets. *Rep. Prog. Phys.* **71**, 036601 (2008).

[26] Kupfer, K., Bers, A. & Ram, A. K. The cusp map in the complex-frequency plane for absolute instabilities. *Phys. Fluids* **30**, 3075–3082 (1987).

[27] Coullet, P., Elphick, C. & Repaux, D. Nature of spatial chaos. *Phys. Rev. Lett.* **58**, 431–434 (1987).

[28] Dee, G. T. & van Saarloos, W. Bistable systems with propagating fronts leading to pattern formation. *Phys. Rev. Lett.* **60**, 2641–2644 (1988).

[29] Rottschäfer, V. & Doelman, A. On the transition from the Ginzburg–Landau equation to the extended Fisher–Kolmogorov equation. *Physica D* **118**, 261–292 (1998).

[30] Cross, M. & Greenside, H. *Pattern Formation and Dynamics in Nonequilibrium Systems* (Cambridge University Press, 2009).

[31] Dee, G. & Langer, J. S. Propagating pattern selection. *Phys. Rev. Lett.* **50**, 383–386 (1983).

[32] Ben-Jacob, E., Brand, H., Dee, G., Kramer, L. & Langer, J. S. Pattern propagation in nonlinear dissipative systems. *Physica D.* **14**, 348–364 (1985).

[33] van Saarloos, W. Front propagation into unstable states. II. Linear versus nonlinear marginal stability and rate of convergence. *Phys. Rev. A* **39**, 6367–6390 (1989).

[34] Bar-Ziv, R., Moses, E. & Nelson, P. Dynamic excitations in membranes induced by optical tweezers. *Biophys. J.* **75**, 294–320 (1998).

[35] Hornreich, R. M., Luban, M. & Shtrikman, S. Critical behavior at the onset of $\vec{k}$-instability on the $\lambda$-line. *Phys. Rev. Lett.* **35**, 1678–1681 (1975).

[36] Kramer, L., Bodenschatz, E., Pesch, W., Thom, W. & Zimmermann, W. New results on the electrohydrodynamic instability in nematics. *Liq. Cryst.* **5**, 699–715 (1989).

[37] Bodenschatz, E., Kaiser, M., Kramer, L., Weber, A. & Zimmermann, W. *Hydrodynamic instabilities in open flows*, 111–124. NATO Advanced Study Institutes Series (Plenum, 1990).

[38] Zimmermann, W. Propagating fronts near a Lifshitz point. *Phys. Rev. Lett.* **50**, 383–386 (1983).

[39] van Saarloos, W. Front propagation into unstable states. *Phys. Rep.* **386**, 29–222 (2009).

[40] Hecht, F. New development in FreeFem++. *J. Numer. Math.* **20**, 251–265 (2012).

[41] Chomaz, J.-M. Fully nonlinear dynamics of parallel wakes. *J. Fluid Mech.* **495**, 57–75 (2003).

[42] Pullarkat, P. A., Dommersnes, P., Fernández, P., Joanny, J.-F. & Ott, A. Osmotically driven shape transformations in axons. *Phys. Rev. Lett.* **96**, 048104 (2006).
